# Supplementary material for: Gyro-based Neural Single Image Deblurring
Source: arXiv:2404.00916 source file (2025-04-04)
Supplement: Supplementary file 1 [file X_suppl.tex]

\clearpage
\maketitlesupplementary
\setcounter{page}{1}
\setcounter{section}{0}
\setcounter{figure}{0}
\setcounter{table}{0}

% 추가할 내용들
% - Gyro synchronization 관련 얘기
% 

\section{Overview}
In the supplementary material, we provide additional analyses, implementation details and additional qualitative results on \SynthDataName{} and \RealDataName{}.
Specifically, we provide:

\begin{itemize}
    \item Network training details
    \item Details on the blur synthesis pipeline
    \item Additional analysis on the effect of our gyro error handling
    %\item Visualization of the effect of gyro refinement
    %\item Analysis on the gyro error robustness
    %\item Result of training NAFNet with gyro data
    \item Details on the datasets
    \item Details on our extension of the non-blind deblurring methods
    \item Network architectures
    \item Additional qualitative results including real-world images with moving objects
\end{itemize}

%Additional analysis on the effect of our gyro error handling
% - Visualization of the effect of gyro refinement
% - Analysis on the gyro error robustness
% - Comparison against a simple extension of an existing non-gyro method

\begin{figure}[t]
\centering
\includegraphics[width=\linewidth]{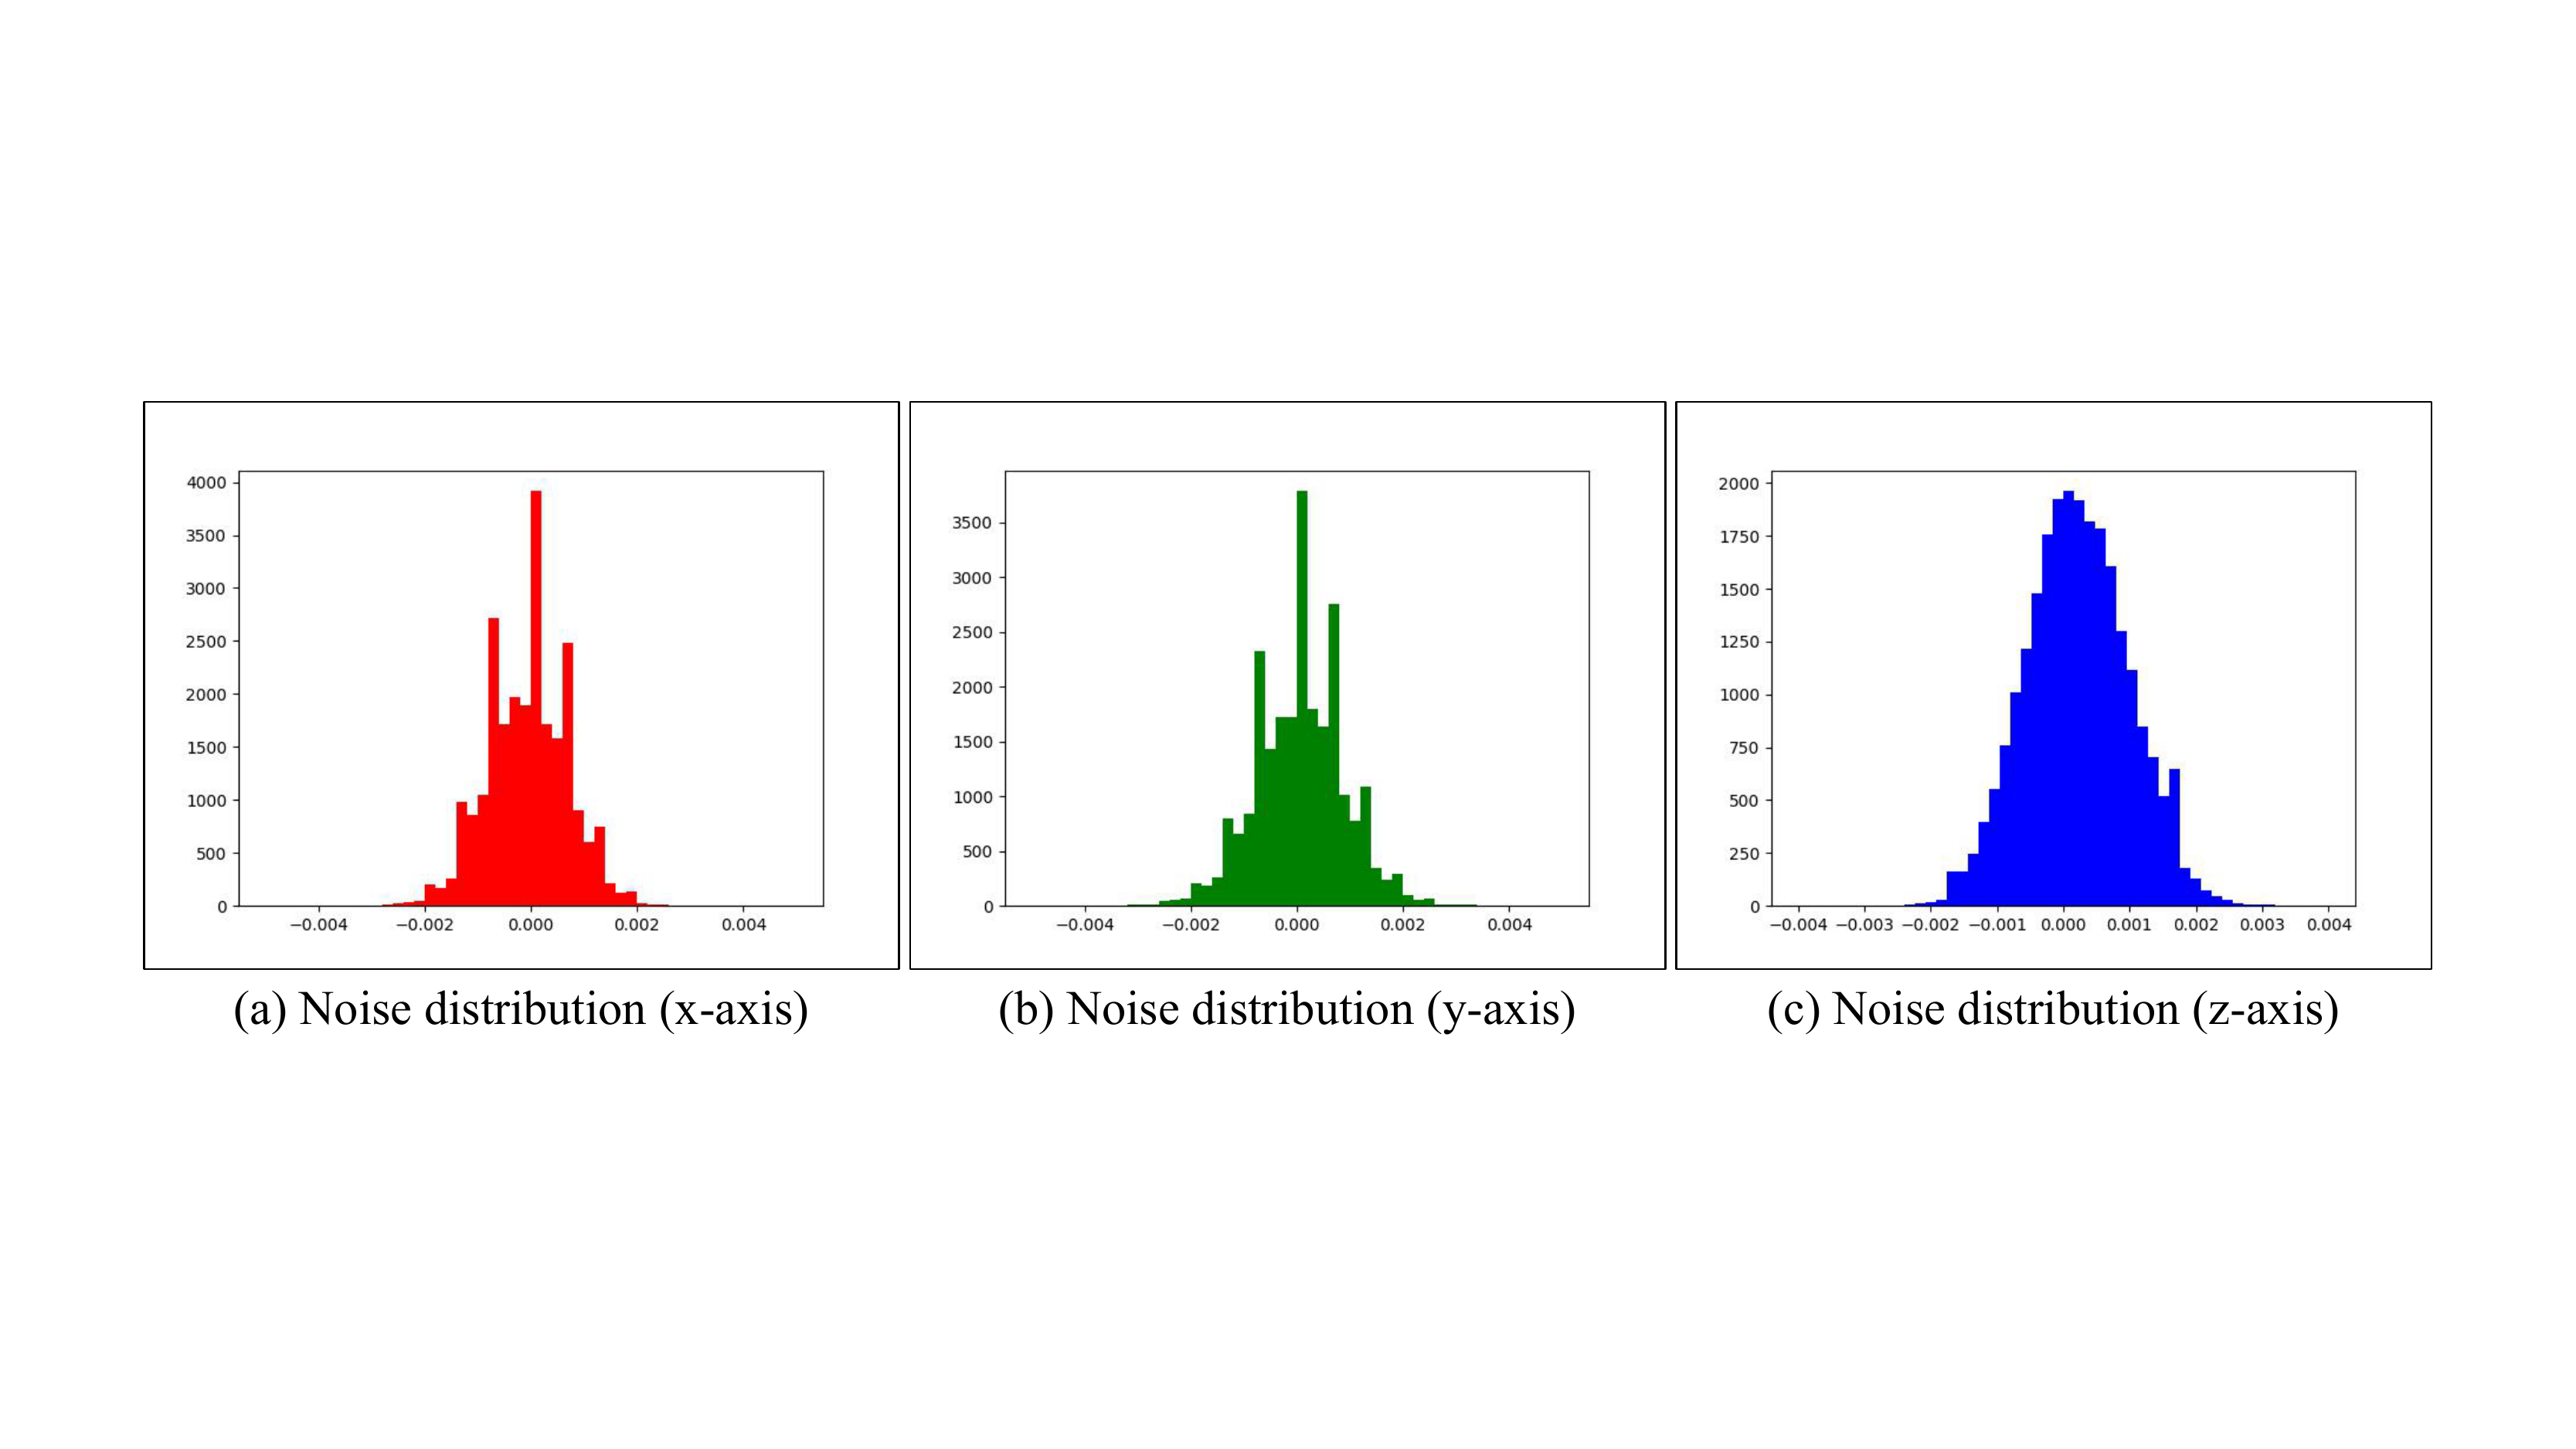}
\caption{Noise distributions of the Galaxy S22 gyro sensor.}
\label{fig:gyro_noise}
\end{figure}

\section{Network Training Details}
\paragraph{Generating erroneous camera motion field}
When generating camera motion fields, we add gyro sensor noise and random rotational center shift to simulate real-world gyro noise.
To measure gyro sensor noise distributions, we placed a Samsung Galaxy S22 smartphone on a stationary table.
We then collected gyro data for 120 seconds and estimated the noise distribution for the $x$, $y$ and $z$ axes respectively.
We found out that noise in the gyro data for each axis follows distinct normal distributions (\cref{fig:gyro_noise}), characterized by their respective means and standard deviations.
The estimated noise distributions are:
\begin{align}
\label{eq:noise_distribution}
    n_x&\sim \mathcal{N}(-0.00005643153, 0.0008631607^2) \\
\label{eq:noise_distribution1}
    n_y&\sim \mathcal{N}(-0.00006369004, 0.0015023947^2) \\
\label{eq:noise_distribution2}
    n_z&\sim \mathcal{N}(0.00021379517, 0.0007655643^2)
\end{align}
where $n_x$, $n_y$ and $n_z$ represent the noise distributions of the $x$, $y$ and $z$ axes, respectively.
The amount of rotational center shift is randomly sampled from $[-500, 500]$ pixels for both $x$ and $y$ axes of the image plane following Hu~\etal~\cite{hu2016gyro}.

\paragraph{Scheduling of $\alpha$}
To apply the curriculum-learning-based training strategy to train our network, we gradually increase $\alpha$ from 0 to 1 during the training.
Our scheduling protocol for $\alpha$ is
\begin{align}
    \alpha = 
    \begin{cases}
        0.1 \cdot \lfloor\, ep/10\, \rfloor & \text{if } ep < 100  \\
        1 & \text{otherwise}
    \end{cases}
\end{align}
where $ep$ denotes the current training epoch.

\begin{table}[t]
    \centering
\scalebox{0.83}{\begin{tabular}{@{\hspace{2mm}}c@{\hspace{2mm}}|@{\hspace{2mm}}c@{\hspace{2mm}}}
\toprule[1.5pt]
Noise parameter                                                        & Value          \\ \midrule
$\log_2(\text{shot noise})$ at ISO 100                                 & -10.0009938243 \\
$\log_2(\text{shot noise})$ at ISO 1600                                & -9.3348824266  \\ 
Slope of $\log_2(\text{shot noise})$ - $\log_2(\text{read noise})$     & 3.15578751     \\
Intercept of $\log_2(\text{shot noise})$ - $\log_2(\text{read noise})$ & 10.0003514152  \\ \bottomrule[1.5pt]
\end{tabular}}
% \vspace{-2mm}
\caption{Noise parameters for RSBlur blur synthesis pipeline.}
\label{table:rsblur_parameter}
\end{table}

\section{Blur Synthesis Pipeline}
As mentioned in our main paper, we adopt the RSBlur pipeline~\cite{rim2022rsblur} to synthesize realistic blurred images in \SynthDataName{}.
Our detailed process to generate the blurry images in \SynthDataName{} is as follows.
For generating each blurry image, we first sample a sharp image and a sequence of gyro data samples, and interpolate the gyro data samples as described in our main paper.
Then, following the RSBlur pipeline, we warp the sharp image using the gyro data samples, convert the color space of the warped sharp images to the linear space, and average them to obtain a blurred image.
We then perform the remaining steps of the RSBlur pipeline including the saturation synthesis, conversion to RAW, noise synthesis, and camera ISP to obtain a realistic blurred image.
Regarding the shot and read noise, we estimate their distributions from a Samsung Galaxy S22 ultra-wide camera, which are reported in \cref{table:rsblur_parameter}.
We refer the readers to \cite{rim2022rsblur} for more details on the blur synthesis process.

% For generating each blurry image in \SynthDataName{}, we 
% Before averaging sharp images to generate blurry images in \SynthDataName{}, we first extract a saturation mask for each blurry image.
% When training the network, we first add corresponding saturation mask to the blurry image and clip the image.
% Then, the image is transformed to CIE XYZ color space and the inverse color correction is applied to the image.
% We then apply inverse white balance by sampling the red channel gain from $[1.9, 2.4]$ and the blue channel gain from $[1.5, 1.9]$ and multiplying the inverse of them to red and blue channels.

% We synthesize noise to the image by randomly sampling shot noise and read noise variances at this step.
% The variances are estimated using flat frames and dark frames that are taken using the same camera.
% We first estimate the noise variances at ISO 100, 200, 400, 800, 1600 and use the linear relationship between $\log_2(\text{shot noise})$ and $\log_2(\text{read noise})$ to randomly sample noise variances each time.
% \cref{table:rsblur_parameter} shows the noise parameters of Samsung Galaxy S22 ultra-wide camera that is used for the blur synthesis pipeline.
% After synthesizing shot noise and read noise, we apply white balance, color correction and conversion from the CIE XYZ color space to the linear sRGB color space.

\begin{figure}[t]
\centering
\includegraphics[width=\linewidth]{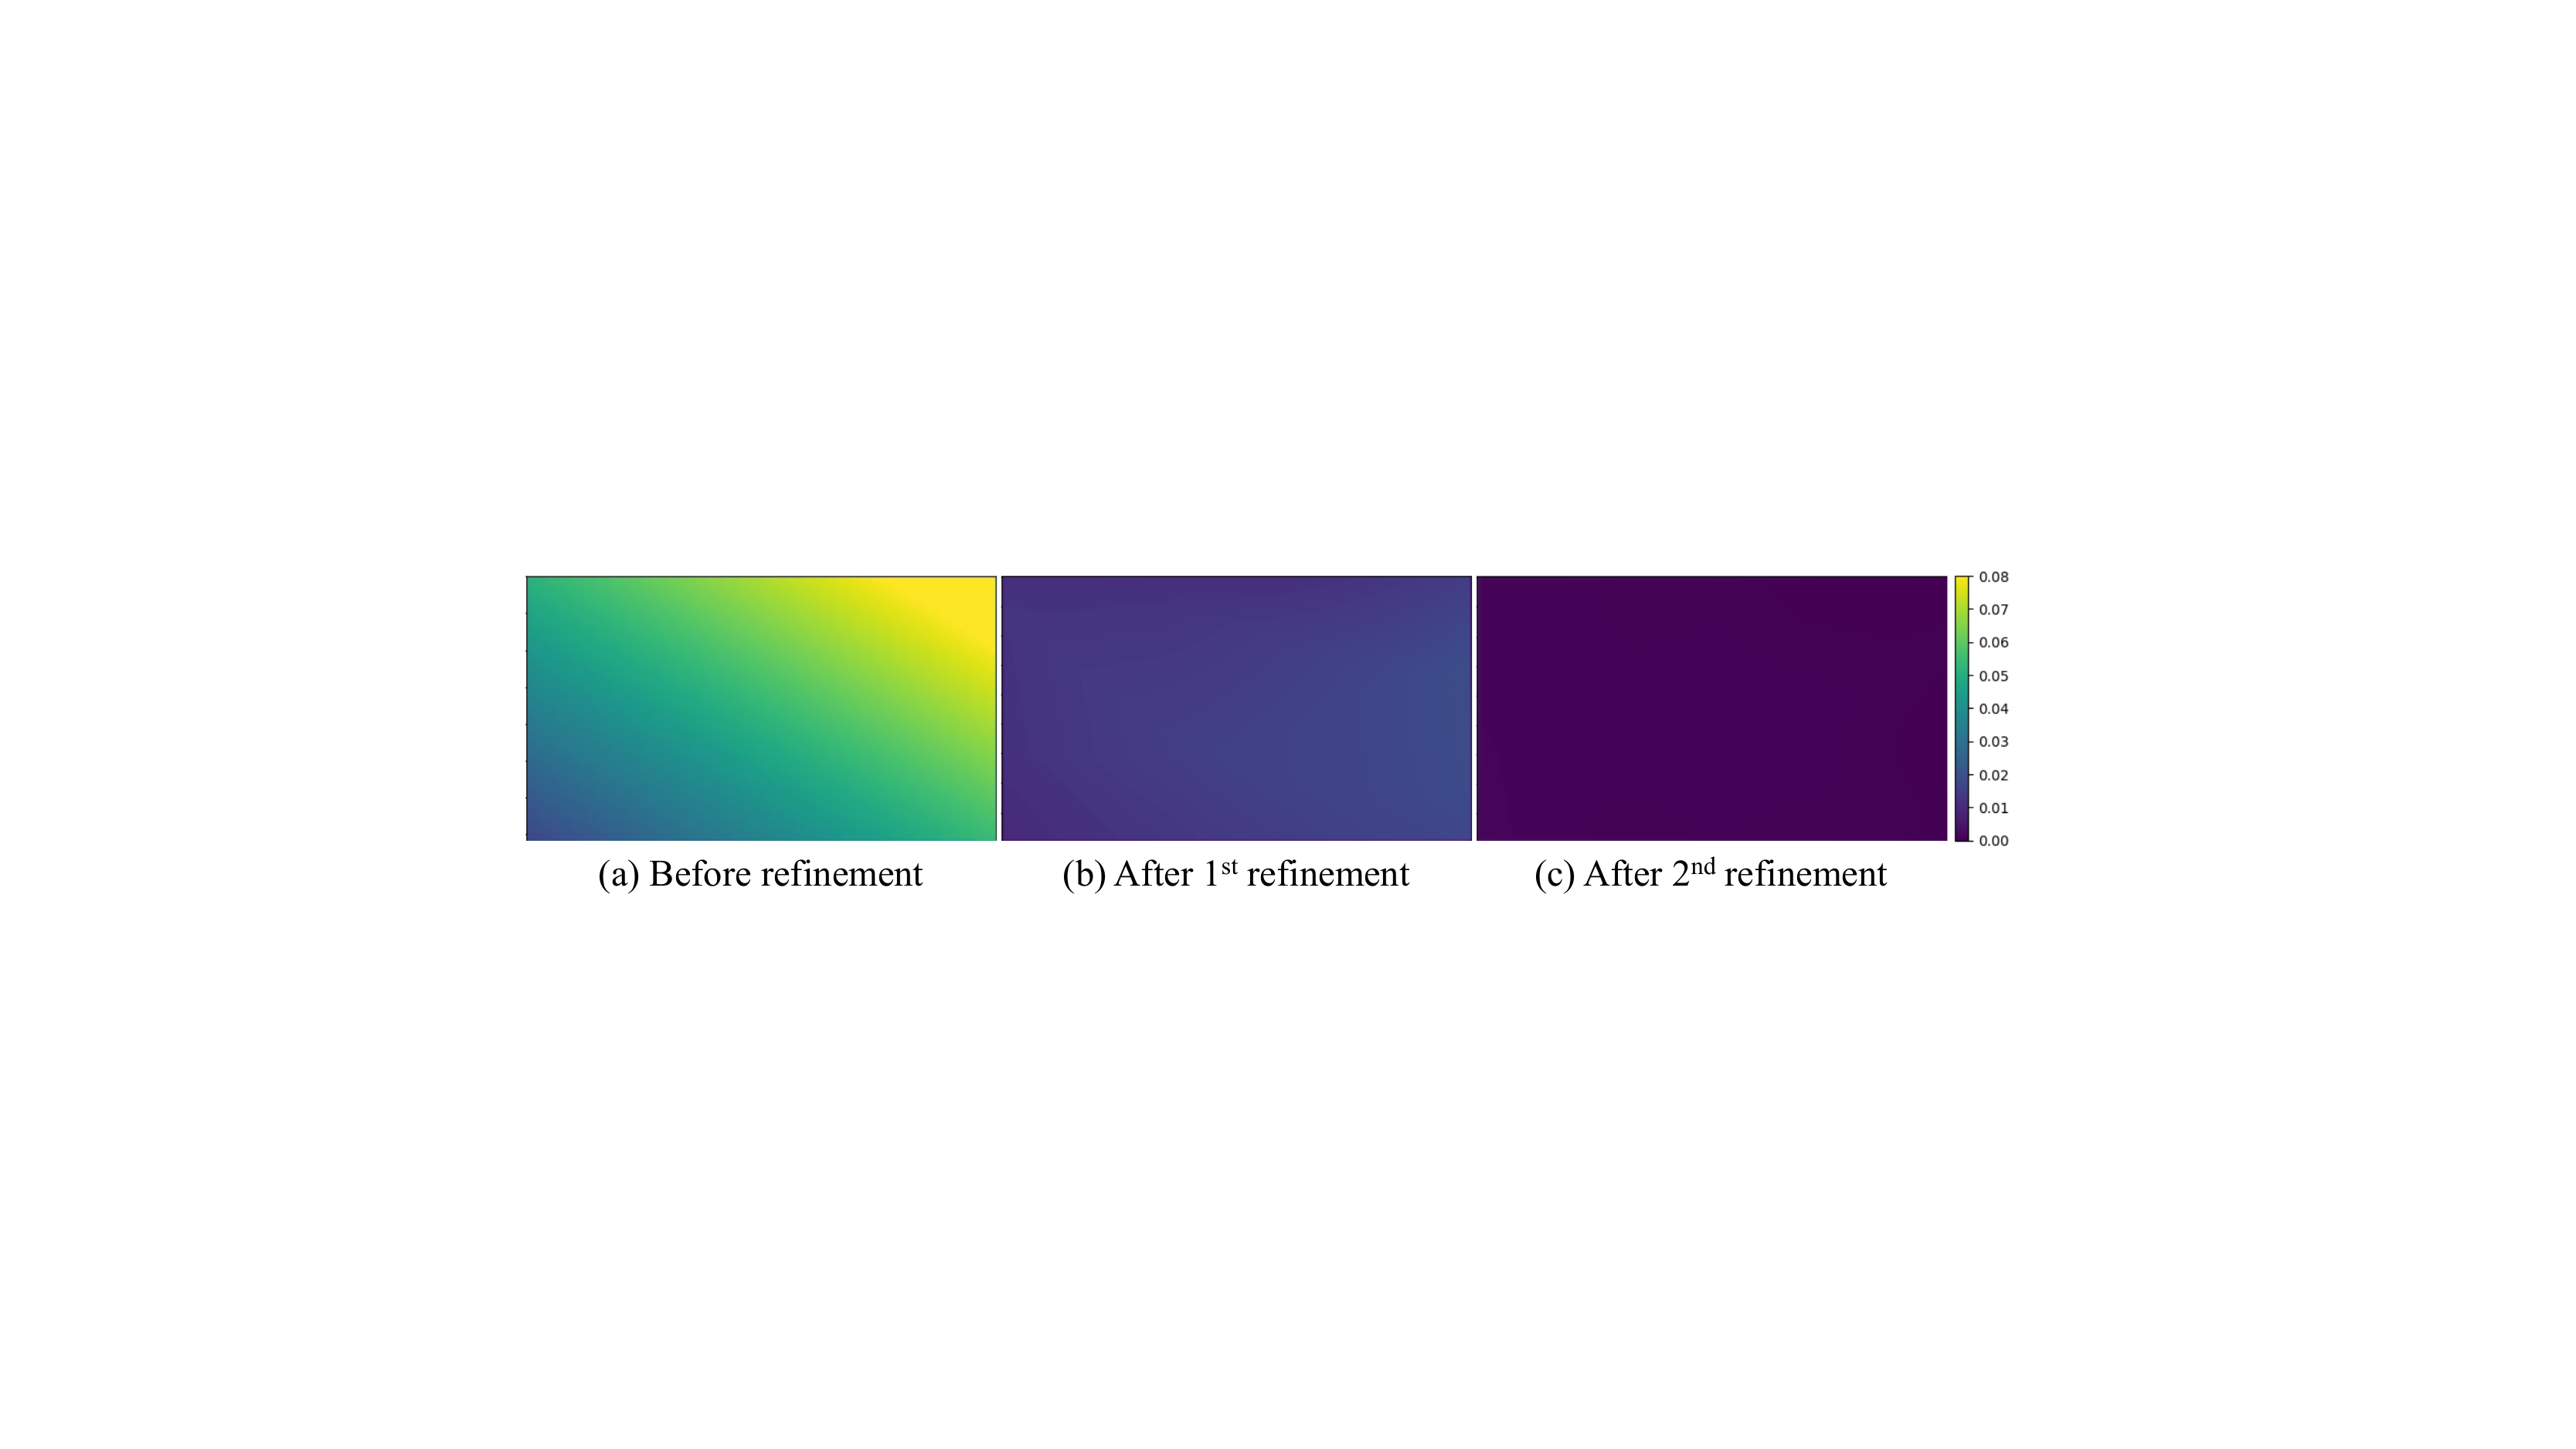}
\caption{Error map between accurate gyro feature map and erroneous gyro feature map for visualizing gyro refinement process. (a) Error map before the gyro refinement blocks. (b) Error map after the first gyro refinement block. (c) Error map after the second gyro refinement block.}
\label{fig:gyro_refinement}
\end{figure}

%Additional analysis on the effect of our gyro error handling
% - Visualization of the effect of gyro refinement
% - Analysis on the gyro error robustness
% - Comparison against a simple extension of an existing non-gyro method

\section{Additional Analysis on the Effect of Our Gyro Error Handling}
\subsection{Visualization of the Effect of Gyro Refinement}
To see the effect of the gyro refinement blocks, we visualize errors in gyro features by computing the difference between the gyro features of erroneous and error-free gyro data in \cref{fig:gyro_refinement}.
While the error map between two gyro features before passing the gyro refinement blocks (\cref{fig:gyro_refinement} (a)) shows large error value, errors get reduced as the erroneous gyro feature passes consecutive gyro refinement blocks (\cref{fig:gyro_refinement} (b) \& (c)).
This result indicates that gyro refinement blocks do help the network to refine erroneous gyro features and extract meaningful motion information from erroneous gyro features.

\begin{figure}[t]
\centering
\includegraphics[width=\linewidth]{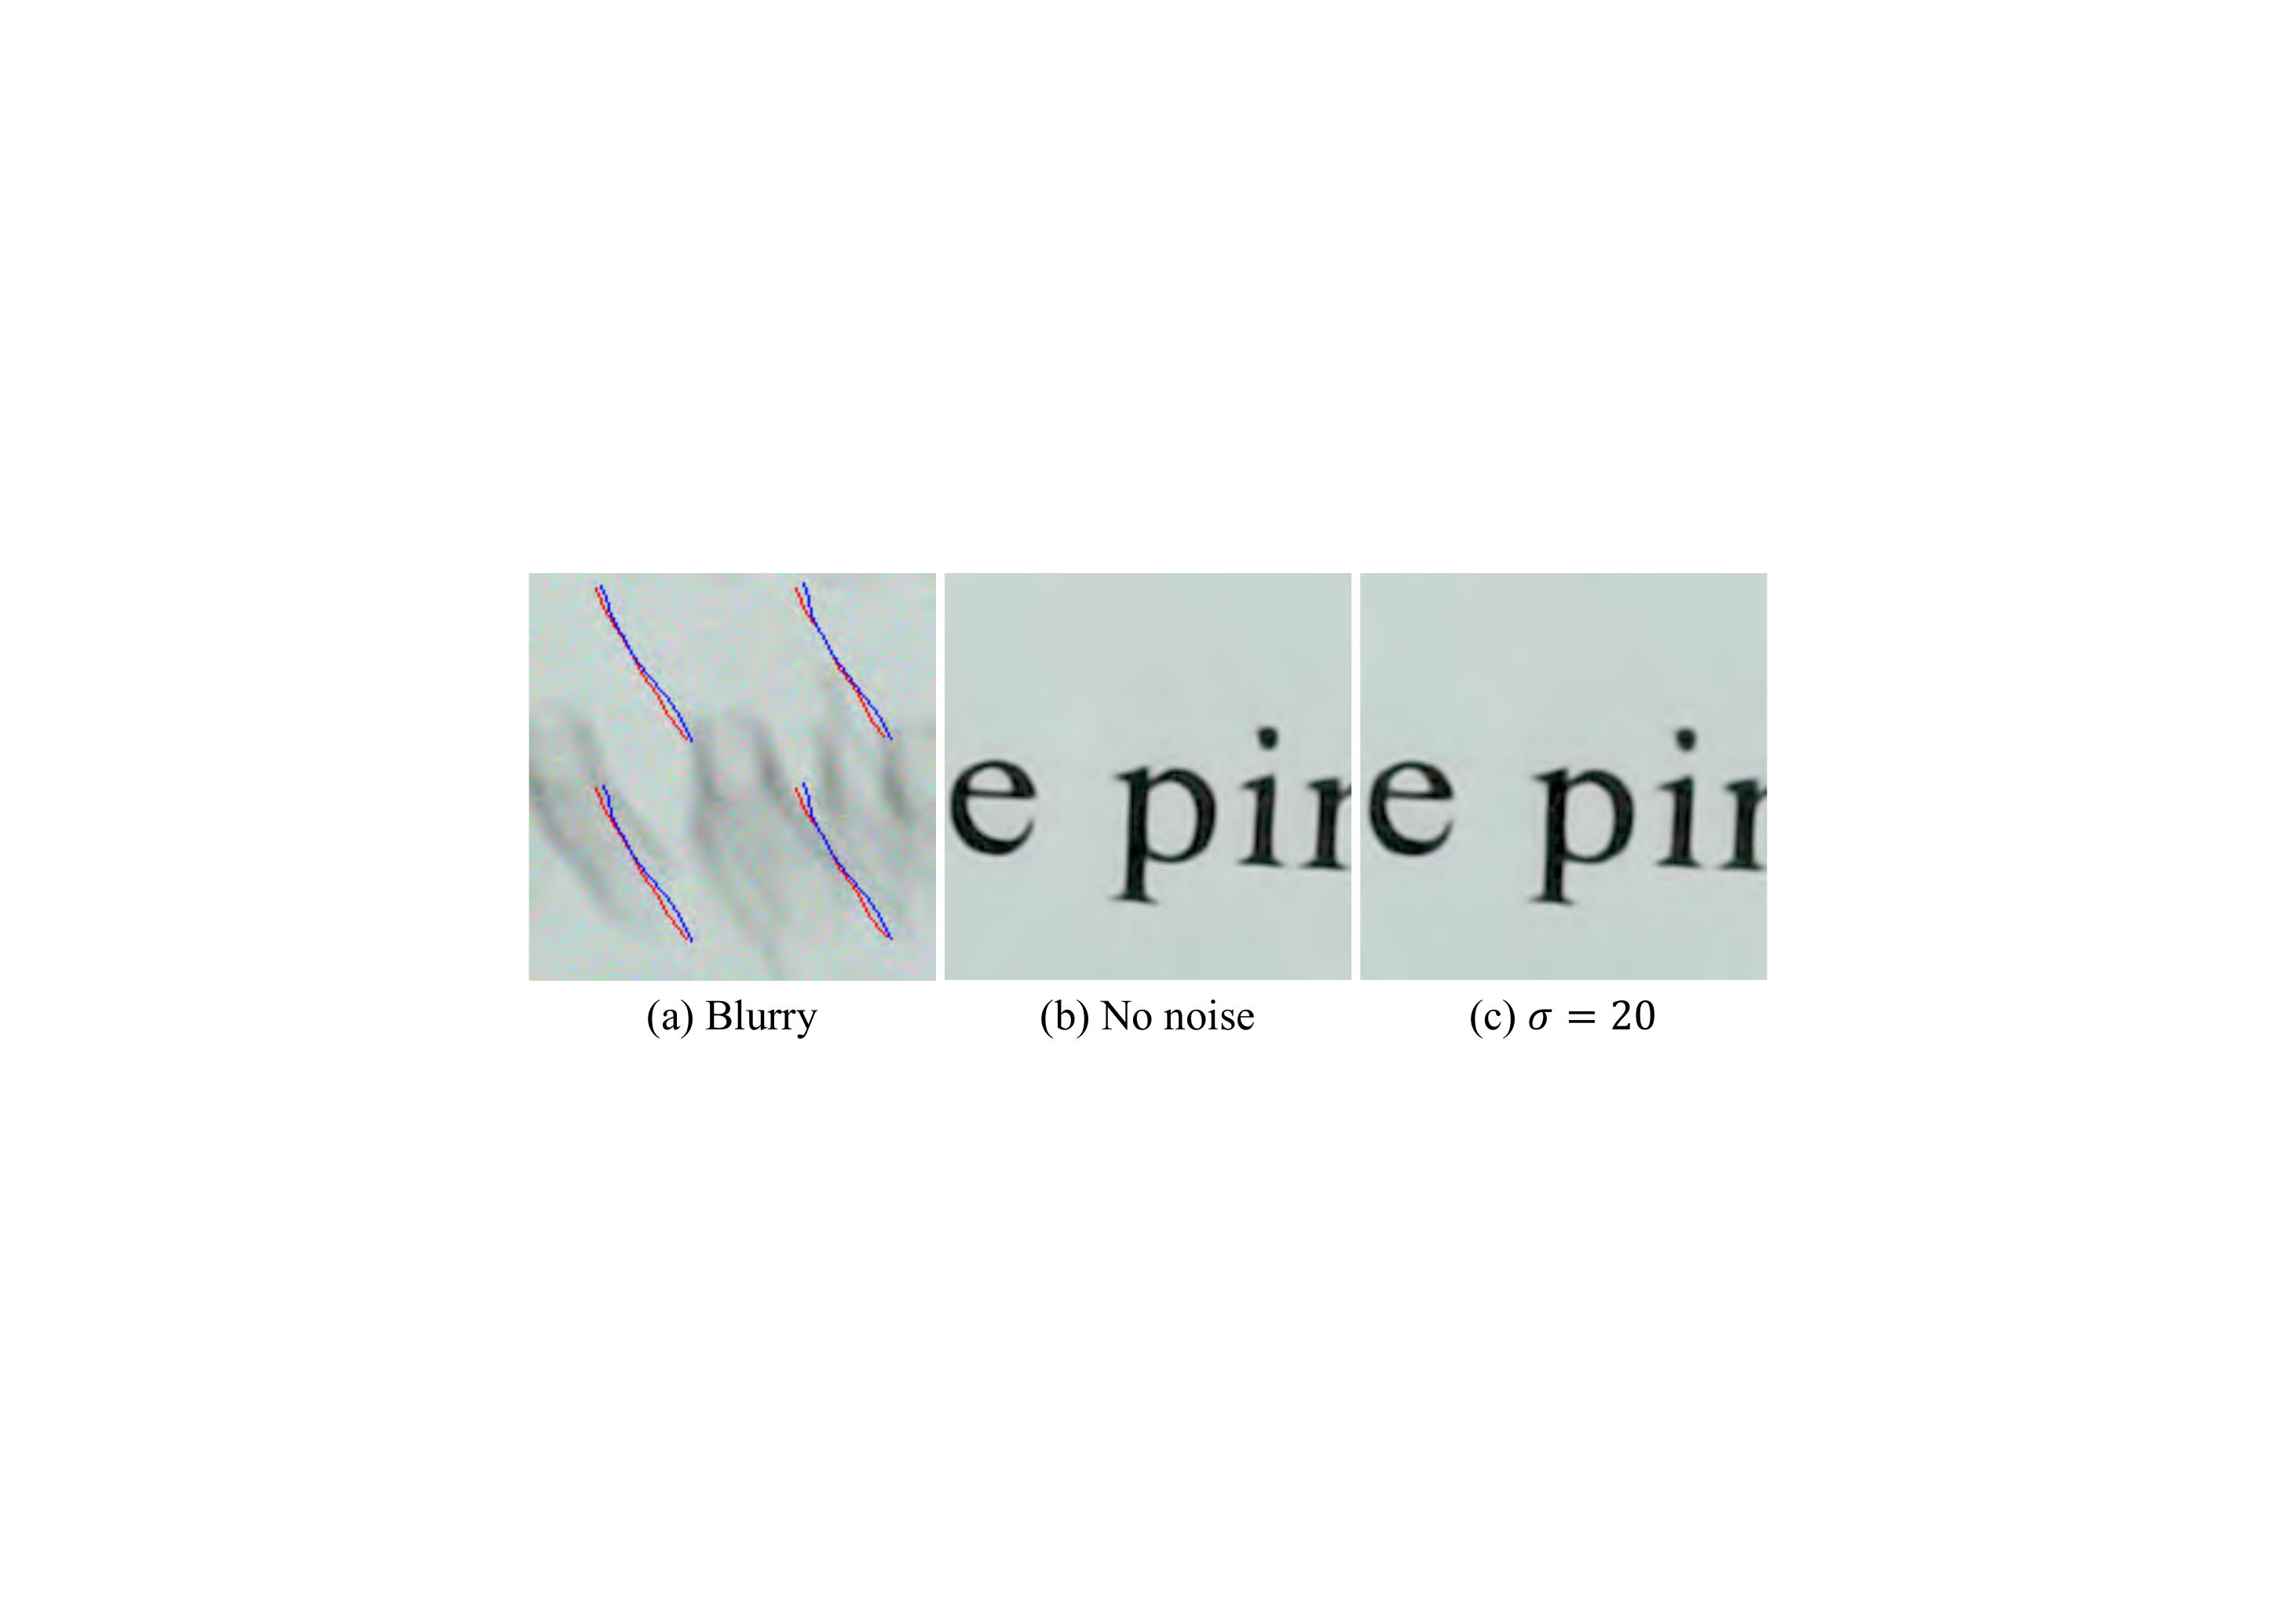}
\caption{Gyro sensor noise visualization. (a) Accurate camera motion field (Blue line) and noisy camera motion field with $\sigma = 20$ (Red line). (b) Deblurred result with accurate camera motion field. (c) Deblurred result with noisy camera motion field.}
\label{fig:noise_visalization}
\end{figure}

\begin{figure}[t]
\centering
\includegraphics[width=\linewidth]{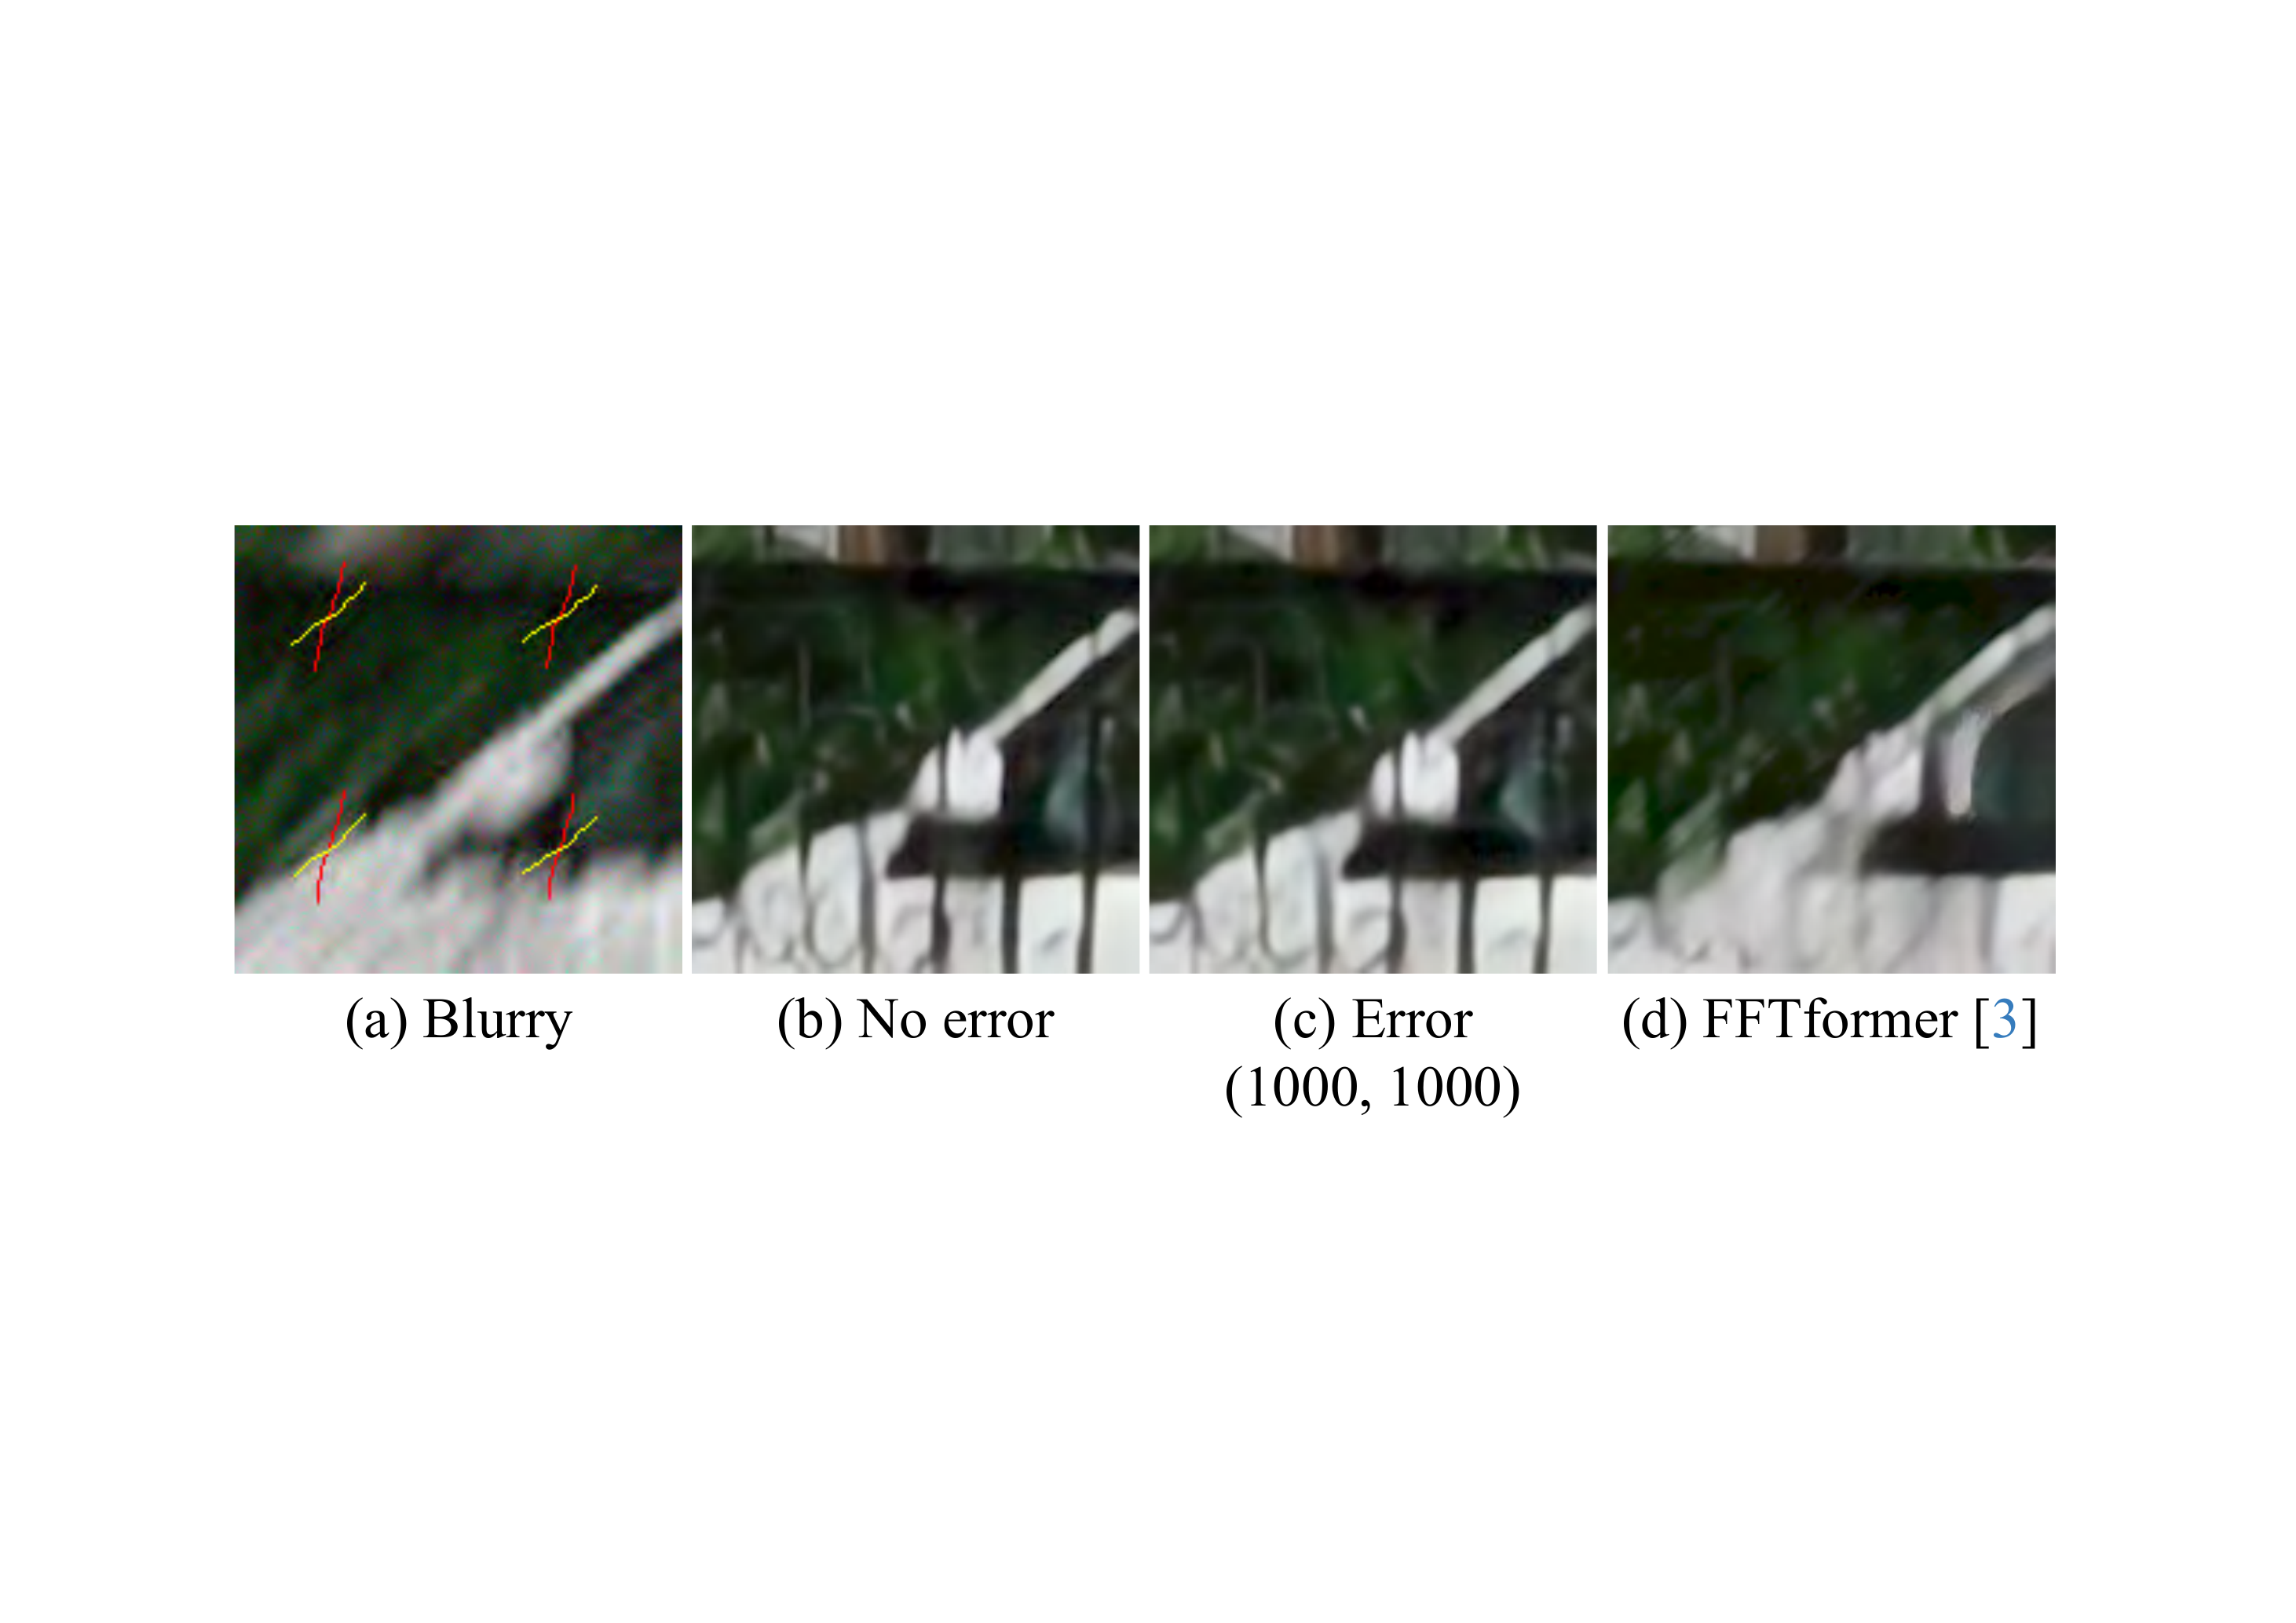}
\caption{Rotational center shift visualization. (a) Accurate camera motion field (Yellow line) and erroneous camera motion field with rotational center error $(1000, 1000)$ (Red line). (b) Deblurred result with the accurate camera motion field. (c) Deblurred result with the erroneous camera motion field. (d) Deblurred result of FFTformer~\cite{kong2023fftformer}.}
\label{fig:rot_cen_visualization}
\end{figure}

\begin{table}[t]
    \centering
    \scalebox{1}{
        \begin{tabular}{@{\hspace{2mm}}c@{\hspace{2mm}}|@{\hspace{2mm}}c@{\hspace{2mm}}c@{\hspace{2mm}}c@{\hspace{2mm}}c@{\hspace{2mm}}c@{\hspace{2mm}}}
            \toprule[1.5pt]
            Noise level & 0      & 5$\sigma$ & 10$\sigma$ & 15$\sigma$ & 20$\sigma$ \\ \midrule
            PSNR        & 27.44  & 27.39     & 27.37      & 27.36      & 27.30      \\
            SSIM        & 0.7850 & 0.7843    & 0.7837     & 0.7838     & 0.7824     \\
            \bottomrule[1.5pt]
        \end{tabular}
    }
\caption{Analysis on robustness to gyro sensor noise. $\sigma$ denotes standard deviation of the noise distribution.}
\label{table:robust_noise}
\end{table}

\begin{table}[t]
    \centering
    \scalebox{0.7}{
        \begin{tabular}{@{\hspace{2mm}}c@{\hspace{2mm}}|@{\hspace{2mm}}c@{\hspace{2mm}}c@{\hspace{2mm}}c@{\hspace{2mm}}c@{\hspace{2mm}}c@{\hspace{2mm}}|@{\hspace{2mm}}c@{\hspace{2mm}}}
            \toprule[1.5pt]
            Max. shift (px.) & 0      & 250    & 500    & 750    & 1000   & FFTformer~\cite{kong2023fftformer} \\ \midrule
            PSNR             & 27.44  & 27.38  & 27.30  & 26.95  & 26.71  & 26.01                              \\
            SSIM             & 0.7850 & 0.7829 & 0.7804 & 0.7705 & 0.7614 & 0.7481                             \\
            \bottomrule[1.5pt]
        \end{tabular}
        % \begin{tabular}{@{\hspace{2mm}}c@{\hspace{2mm}}|@{\hspace{2mm}}c@{\hspace{2mm}}c@{\hspace{2mm}}}
        %     \Xhline{4\arrayrulewidth}
        %     Max. shift (px.) & PSNR  & SSIM   \\ \hline 
        %     0                & 27.44 & 0.7850 \\
        %     250              & 27.38 & 0.7829 \\
        %     500              & 27.30 & 0.7804 \\
        %     750              & 26.83 & 0.7697 \\
        %     1000             & 26.44 & 0.7518 \\ \hline
        %     FFTformer~\cite{kong2023fftformer} & 26.01 & 0.7481 \\
        %     \Xhline{4\arrayrulewidth}
        % \end{tabular}
    }
\caption{Analysis on robustness to rotational center shift.}
\label{table:robust_rotational_center_shift}
\end{table}

\subsection{Robustness to Gyro Error}
In this section, we analyze the robustness of our method to gyro error.
To this end, we construct camera motion field variants with different amounts of gyro errors.
We analyze the error robustness with two gyro error sources, which are gyro sensor noise and rotational center shift.
\cref{table:robust_noise} and \cref{table:robust_rotational_center_shift} show quantitative results of \MethodName{} on \SynthDataName{} with different amount of gyro errors.
\cref{table:robust_noise} shows the result of \MethodName{} with different noise level.
In the table, $\sigma$ denotes the standard deviation of noise distributions given in \cref{eq:noise_distribution}, \cref{eq:noise_distribution1} and \cref{eq:noise_distribution2}.
To see the robustness to the noise only, rotational center shift errors are not considered. % the camera motion fields.
\cref{table:robust_rotational_center_shift} shows the results of \MethodName{} with different amounts of rotational center shift.
Similarly, we do not consider gyro sensor noise to see the robustness to the rotational center shift only.

As shown in \cref{table:robust_noise}, \MethodName{} shows strong robustness to the gyro sensor noise.
The results show that \MethodName{} can be applied to sensor data with higher sensor noise without severe performance degradation. %, e.g. accelerometer.
\cref{fig:noise_visalization} demonstrates the robustness of our method to high gyro sensor noise.
\cref{table:robust_rotational_center_shift} shows that model performance gradually decreases as the amount of rotational center shift increases.
However, we can also observe that \MethodName{} can utilize gyro data with large rotational center shift, e.g. 1000 pixels, by showing better performance than FFTformer~\cite{kong2023fftformer} even though it is trained with gyro data whose rotational center shifts are sampled from $\left[ -500, 500 \right]$.
\cref{fig:rot_cen_visualization} shows the robustness of our method to large rotational center error compared to FFTformer~\cite{kong2023fftformer}.

\begin{table}[t]
    \centering
\scalebox{1}{\begin{tabular}{@{\hspace{2mm}}c@{\hspace{2mm}}l@{\hspace{2mm}}|@{\hspace{2mm}}c@{\hspace{2mm}}c@{\hspace{2mm}}}
\toprule[1.5pt]
    & Model                            & PSNR  & SSIM   \\ \midrule
(a) & NAFNet~\cite{chen2022nafnet}     & 25.06 & 0.7085 \\
(b) & NAFNet + Camera motion field     & 24.57 & 0.6802 \\ 
(c) & (b) + Curriculum learning        & 24.61 & 0.6813 \\ 
(d) & Ours without curriculum learning & 26.94 & 0.7667 \\
(e) & Ours with curriculum learning    & 27.28 & 0.7803 \\ \bottomrule[1.5pt]
\end{tabular}}
\caption{Result of training NAFNet with the concatenation of camera motion fields and blurry images.}
\label{table:nafnet_with_gyro}
\end{table}

\subsection{Comparison against a Simple Extension of an Existing Non-gyro Method}
As our approach exploits additional gyro data to deblur an image, one may wonder whether na\"ively adopting gyro data would improve the performance of existing non-gyro-based deblurring networks.
Here we argue that our gyro error handling schemes including the gyro refinement and gyro deblurring blocks are crucial for effectively handling real-world gyro data, and na\"ively extending a non-gyro-based method to use gyro data results in performance degradation rather than improvement.

To verify this, we conduct an experiment where we extend NAFNet~\cite{chen2021hinet}, which is one of the non-gyro-based state-of-the-art deblurring networks, to use gyro data. Specifically, we change the first layer of NAFNet to take a concatenation of a blurred image and a camera motion field as input.
Note that the modified NAFNet model takes a camera motion field of the same spatial size as the blurred image unlike \MethodName{} that takes a downsampled camera motion field.
We then train the modified NAFNet model using the training set of \SynthDataName{} with and without curriculum learning, and evaluate its performance on the test set of \SynthDataName{}.

\cref{table:nafnet_with_gyro} shows the evaluation result.
As the table shows, the modified NAFNet (\cref{table:nafnet_with_gyro}-(b)) achieves lower PSNR and SSIM scores than the original NAFNet model despite using additional gyro data, and the curriculum learning-based training strategy does not help the model to achieve noticeable performance gain (\cref{table:nafnet_with_gyro}-(c)).
However, our method without curriculum learning achieves significantly higher PSNR and SSIM scores (\cref{table:nafnet_with_gyro}-(d)) compared to the na\"ive extension of NAFNet, and our curriculum learning scheme further enhances the performance (\cref{table:nafnet_with_gyro}-(e)).
This result proves that na\"ive extension of a non-gyro method cannot handle erroneous gyro data, and that our gyro error handling scheme is crucial for handling real-world gyro data.

\section{Dataset Details}
\paragraph{Synthesizing moving objects}
We synthesize moving objects by randomly sampling moving directions and distances.
When synthesizing a blurred image with a moving object, we first randomly sample the direction of the moving object from $[0^\circ,360^\circ)$.
Then, we sample the moving distance of the object from the range of 30 to 70 pixels.

\paragraph{Post-processing \RealDataName{}}
\RealDataName{} provides both JPEG and raw DNG images.
Nevertheless, in our evaluations using \RealDataName{} in our paper, we use only raw DNG images.
As our network requires 3-channel images, in our evaluation, we first demosaicked raw DNG images to use them.
For demosaicking, we used the \texttt{postprocess()} function of the Python \texttt{rawpy} package.

\paragraph{Synchronization between the gyro sensor and the camera}
One well-known issue in using gyro data is that the timestamps of the gyro sensor and the camera are not synchronized.
To resolve the issue when collecting the \RealDataName{} dataset, we used the Android API that supports synchronization between the gyro sensor and the camera.
Specifically, we used the Camera ITS test\footnote{https://source.android.com/docs/compatibility/cts/camera-its-tests?\#test\_sensor\_fusion} provided by Android API to find the temporal offset between the camera and the gyro sensor at each capture.
After finding the temporal offset, we used the temporal offset to compensate the temporal misalignment between the camera and the gyro sensor.

\section{Extension of the Non-Blind Deblurring Methods}
We compared our method with non-blind deblurring approaches that are designed to handle kernel errors~\cite{nan2020nonblinderror, vasu2018nonblinderror}.
Since they are designed for uniform blur, we extended them to handle non-uniform blur cases.
Specifically, for the method of Vasu \etal~\cite{vasu2018nonblinderror}, we implemented a non-blind deblurring method for non-uniform blur~\cite{harmeling2010space}.
To apply the implemented non-blind deblurring method to the \SynthDataName{} dataset, we converted the gyro data into patch-wise blur kernels where the size of the kernels is $160 \times 160$ with 50\% overlapping area.
Then, we deblurred each image in the training set of \SynthDataName{} with regularization strengths 0.001, 0.002, 0.005 and 0.01 and trained the neural network of the method with the concatenation of the deblurred images.

For the method of Nan \etal~\cite{nan2020nonblinderror}, we first converted the blurry images into patches whose sizes are $160 \times 160$ with 50\% overlapping area.
Similarly, we converted the gyro data into patch-wise blur kernels whose sizes are $160 \times 160$ with 50\% overlapping area.
Then, we applied the method of Nan \etal~\cite{nan2020nonblinderror} to each patch and alpha-blended the results to generate full-resolution results.

\begin{table}[t]
    \centering
    \scalebox{1.0}{
        \begin{tabular}{@{\hspace{2mm}}c@{\hspace{2mm}}c@{\hspace{2mm}}c@{\hspace{2mm}}c@{\hspace{2mm}}c@{\hspace{2mm}}c@{\hspace{2mm}}}
            \toprule[1.5pt]
            Layer   & Input ch. & Output ch. & Kernel         & Stride & Padding \\ \midrule
            Concat. & c, c      & 2c         & -              & -      & -       \\
            GAP     & 2c        & 2c         & -              & -      & -       \\
            Conv1   & 2c        & c          & 1\,$\times$\,1 & 1      & 0       \\ 
            Mul.    & c         & c          & -              & -      & -       \\
            Conv2   & c         & c          & 3\,$\times$\,3 & 1      & 1       \\
            \bottomrule[1.5pt]
        \end{tabular}
    }
\caption{Detailed architecture of the gyro refinement block. GAP denotes global average pooling operation.}
\label{table:gyro_refinement_block}
\end{table}

\begin{table}[t]
    \centering
    \scalebox{0.9}{
        \begin{tabular}{@{\hspace{2mm}}c@{\hspace{2mm}}c@{\hspace{2mm}}c@{\hspace{2mm}}c@{\hspace{2mm}}c@{\hspace{2mm}}c@{\hspace{2mm}}}
            \toprule[1.5pt]
            Layer         & Input ch. & Output ch. & Kernel         & Stride & Padding \\ \midrule
            Concat.       & 256, 256  & 512        & -              & -      & -       \\
            Conv1         & 512       & 18         & 3\,$\times$\,3 & 1      & 1       \\
            Deform. conv. & 256       & 256        & 3\,$\times$\,3 & 1      & 1       \\ 
            Spatial attn. & 256       & 256        & -              & -      & -       \\
            NAFBlock      & 256       & 256        & -              & -      & -       \\
            Concat.       & 256, 256  & 512        & -              & -      & -       \\
            Conv2         & 512       & 256        & 3\,$\times$\,3 & 1      & 1       \\ 
            \bottomrule[1.5pt]
        \end{tabular}
    }
\caption{Detailed architecture of the gyro deblurring block.}
\label{table:gyro_deblurring_block}
\end{table}

\begin{table}[t]
    \centering
    \scalebox{1.0}{
        \begin{tabular}{@{\hspace{2mm}}c@{\hspace{2mm}}c@{\hspace{2mm}}c@{\hspace{2mm}}c@{\hspace{2mm}}c@{\hspace{2mm}}c@{\hspace{2mm}}}
            \toprule[1.5pt]
            Layer & Input ch. & Output ch. & Kernel         & Stride & Padding \\ \midrule
            Conv1 & 16        & 64         & 3\,$\times$\,3 & 1      & 1       \\
            GRB1  & 64        & 64         & -              & -      & -       \\
            Conv2 & 64        & 128        & 3\,$\times$\,3 & 2      & 1       \\
            GRB2  & 128       & 128        & -              & -      & -       \\
            Conv3 & 128       & 256        & 3\,$\times$\,3 & 2      & 1       \\ \bottomrule[1.5pt]
        \end{tabular}
    }
\caption{Detailed network architecture of gyro module. GRB denotes the gyro refinement block.}
\label{table:gyro_module}
\end{table}

\begin{table}[t]
    \centering
    \scalebox{0.90}{
        \begin{tabular}{@{\hspace{2mm}}c@{\hspace{2mm}}c@{\hspace{2mm}}c@{\hspace{2mm}}c@{\hspace{2mm}}c@{\hspace{2mm}}c@{\hspace{2mm}}}
            \toprule[1.5pt]
            Layer         & Input ch. & Output ch. & Kernel         & Stride & Padding \\ \midrule
            Conv1         & 3         & 32         & 3\,$\times$\,3 & 1      & 1       \\ 
            NAFBlock1\_1  & 32        & 32         & -              & -      & -       \\
            NAFBlock1\_2  & 32        & 32         & -              & -      & -       \\
            Conv2         & 32        & 64         & 2\,$\times$\,2 & 2      & 0       \\ 
            NAFBlock2\_1  & 64        & 64         & -              & -      & -       \\
            NAFBlock2\_2  & 64        & 64         & -              & -      & -       \\
            Conv3         & 64        & 128        & 2\,$\times$\,2 & 2      & 0       \\ 
            NAFBlock3\_1  & 128       & 128        & -              & -      & -       \\
            NAFBlock3\_2  & 128       & 128        & -              & -      & -       \\
            Conv4         & 128       & 256        & 2\,$\times$\,2 & 2      & 0       \\ 
            NAFBlock4\_1  & 256       & 256        & -              & -      & -       \\
            NAFBlock4\_2  & 256       & 256        & -              & -      & -       \\ 
            NAFBlock4\_3  & 256       & 256        & -              & -      & -       \\
            NAFBlock4\_4  & 256       & 256        & -              & -      & -       \\
            GDB1          & 256, 256  & 256        & -              & -      & -       \\ 
            NAFBlock4\_5  & 256       & 256        & -              & -      & -       \\
            NAFBlock4\_6  & 256       & 256        & -              & -      & -       \\ 
            NAFBlock4\_7  & 256       & 256        & -              & -      & -       \\
            NAFBlock4\_8  & 256       & 256        & -              & -      & -       \\
            GDB2          & 256, 256  & 256        & -              & -      & -       \\ 
            NAFBlock4\_9  & 256       & 256        & -              & -      & -       \\
            NAFBlock4\_10 & 256       & 256        & -              & -      & -       \\ 
            NAFBlock4\_11 & 256       & 256        & -              & -      & -       \\
            NAFBlock4\_12 & 256       & 256        & -              & -      & -       \\
            GDB3          & 256, 256  & 256        & -              & -      & -       \\ 
            NAFBlock4\_13 & 256       & 256        & -              & -      & -       \\
            NAFBlock4\_14 & 256       & 256        & -              & -      & -       \\ 
            NAFBlock4\_15 & 256       & 256        & -              & -      & -       \\
            NAFBlock4\_16 & 256       & 256        & -              & -      & -       \\
            Conv5         & 256       & 512        & 1\,$\times$\,1 & 1      & 0       \\
            PixelShuffle  & 512       & 128        & -              & -      & -       \\
            Add           & 128, 128  & 128        & -              & -      & -       \\
            NAFBlock5     & 128       & 128        & -              & -      & -       \\
            Conv6         & 128       & 256        & 1\,$\times$\,1 & 1      & 0       \\
            PixelShuffle  & 256       & 64         & -              & -      & -       \\
            Add           & 64, 64    & 64         & -              & -      & -       \\
            NAFBlock6     & 64        & 64         & -              & -      & -       \\
            Conv7         & 64        & 128        & 1\,$\times$\,1 & 1      & 0       \\
            PixelShuffle  & 128       & 32         & -              & -      & -       \\
            Add           & 32, 32    & 32         & -              & -      & -       \\
            NAFBlock7     & 32        & 32         & -              & -      & -       \\
            Conv8         & 32        & 3          & -              & -      & -       \\
            Add           & 3, 3      & 3          & -              & -      & -       \\ 
            \bottomrule[1.5pt]
        \end{tabular}
    }
\caption{Detailed network architecture of image deblurring module. GDB denotes the gyro deblurring block.}
\label{table:image_deblurring_module}
\end{table}

\section{Network Architecture}
\cref{table:gyro_refinement_block}, \cref{table:gyro_deblurring_block}, \cref{table:gyro_module} and \cref{table:image_deblurring_module} show detailed architectures of the gyro refinement block, gyro deblurring block, gyro module and image deblurring module respectively.

\section{Additional Qualitative Results}
\cref{fig:qualitative_synth_supple_1}, \cref{fig:qualitative_synth_supple_2}, \cref{fig:qualitative_synth_supple_3} and \cref{fig:qualitative_synth_supple_4} show additional qualitative results on \SynthDataName{}. % with full frame.
\cref{fig:qualitative_real_supple_1}, \cref{fig:qualitative_real_supple_2}, \cref{fig:qualitative_real_supple_3} show additional qualitative results on \RealDataName{}-S.
\cref{fig:moving_object_real_supple} shows additional qualitative results on real-world images with moving objects.
We show our additional qualitative results with the results of Stripformer~\cite{Tsai2022Stripformer}, FFTformer~\cite{kong2023fftformer}, EggNet~\cite{ji2021eggnet} for comparison.

\begin{figure*}[t]
\centering
\includegraphics[width=\linewidth]{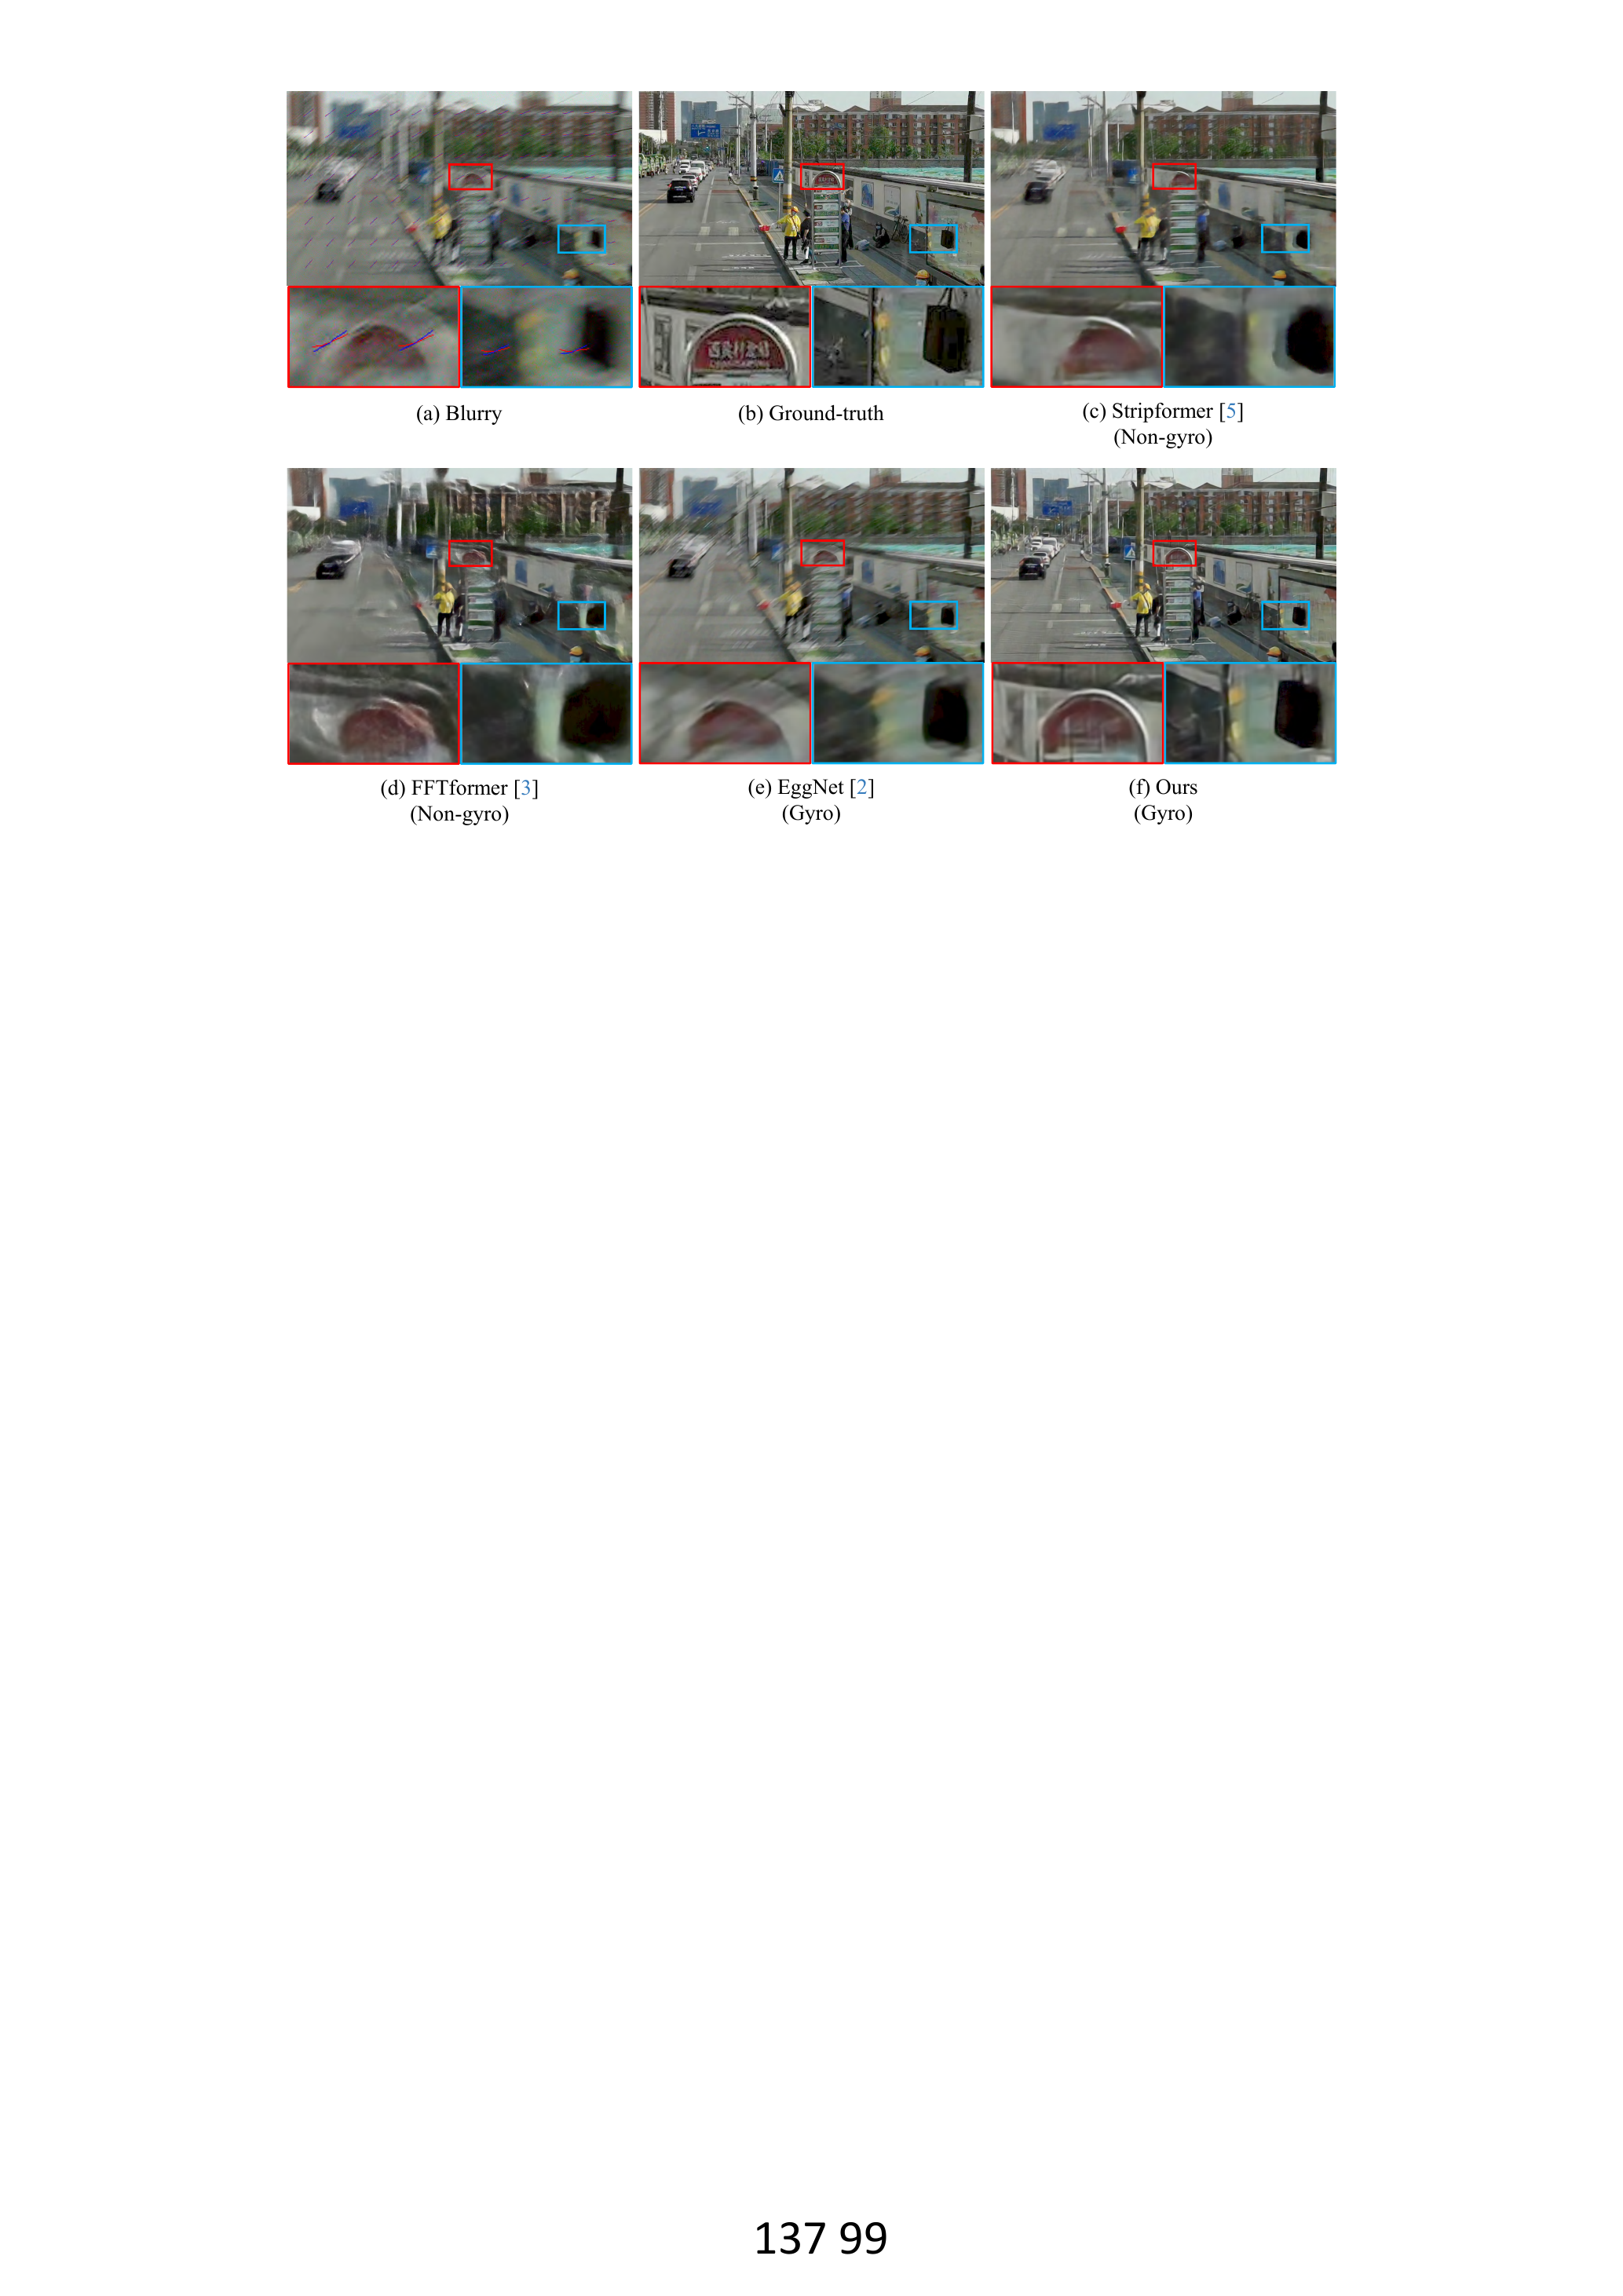}
\caption{Additional qualitative results on \SynthDataName{}. In (a), red lines and blue lines visualize erroneous camera motion field and accurate camera motion field respectively.}
\label{fig:qualitative_synth_supple_1}
\end{figure*}

\begin{figure*}[t]
\centering
\includegraphics[width=\linewidth]{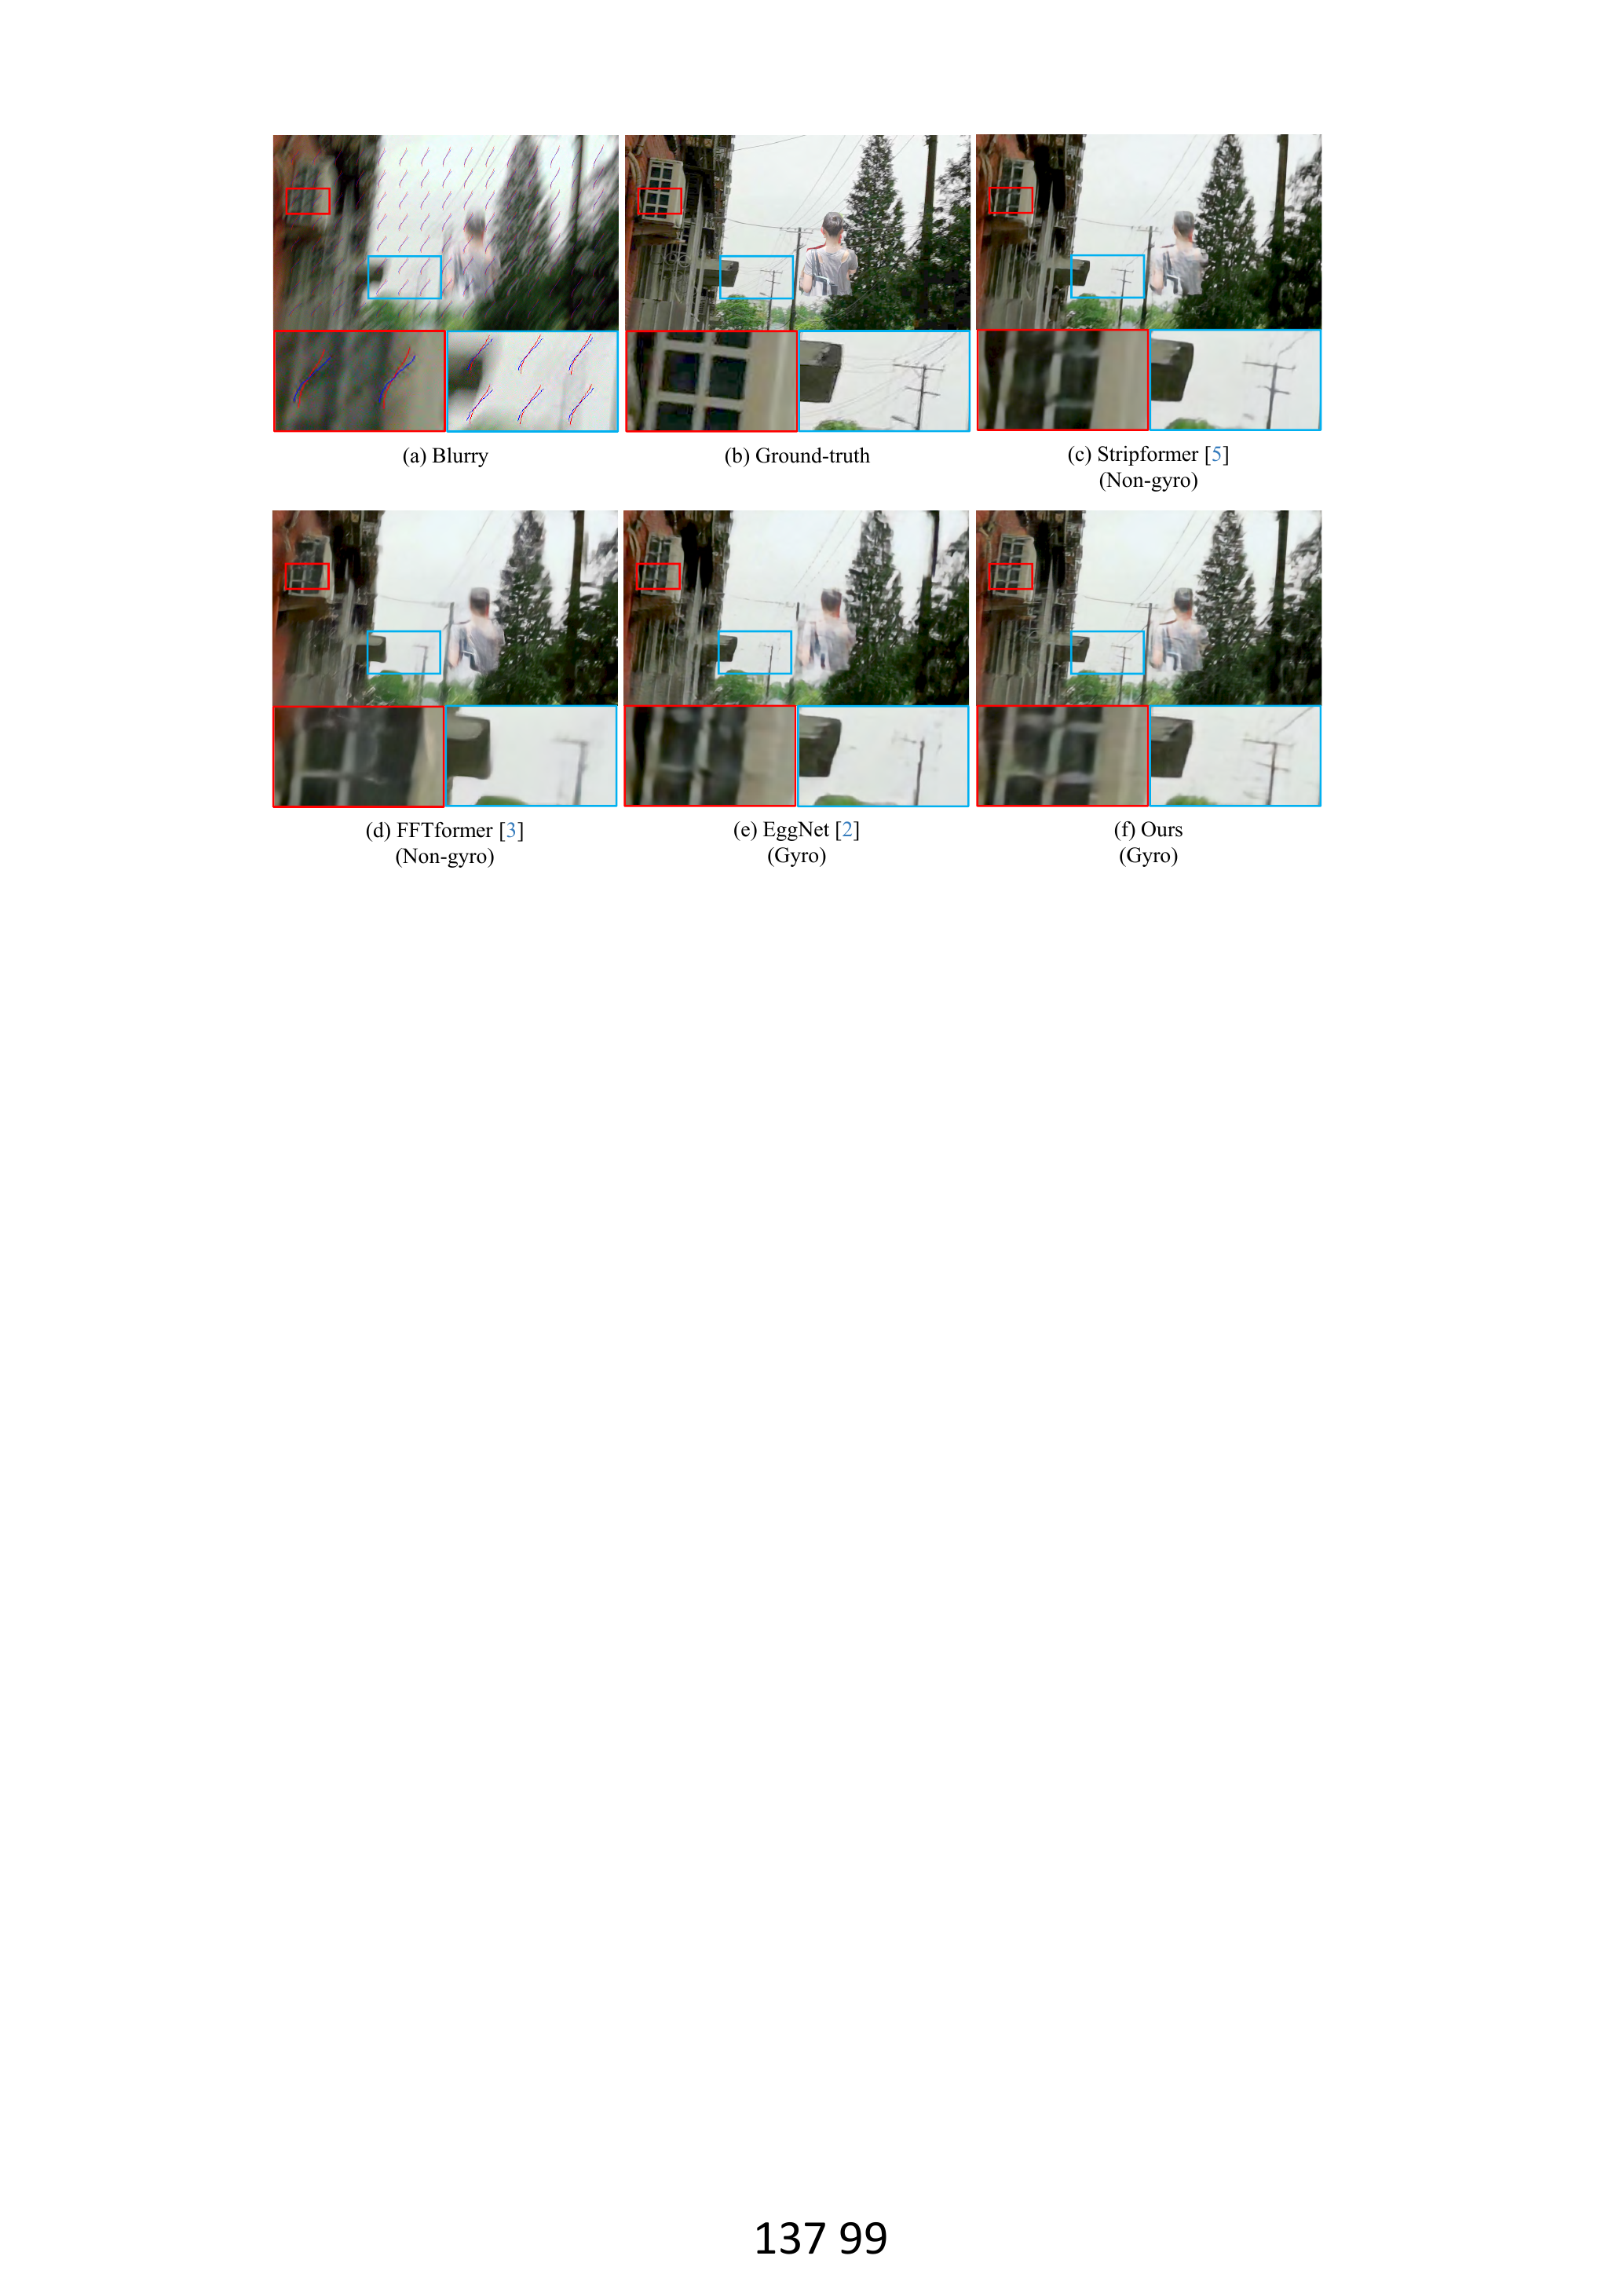}
\caption{Additional qualitative results on \SynthDataName{}. In (a), red lines and blue lines visualize erroneous camera motion field and accurate camera motion field respectively.}
\label{fig:qualitative_synth_supple_2}
\end{figure*}

\begin{figure*}[t]
\centering
\includegraphics[width=\linewidth]{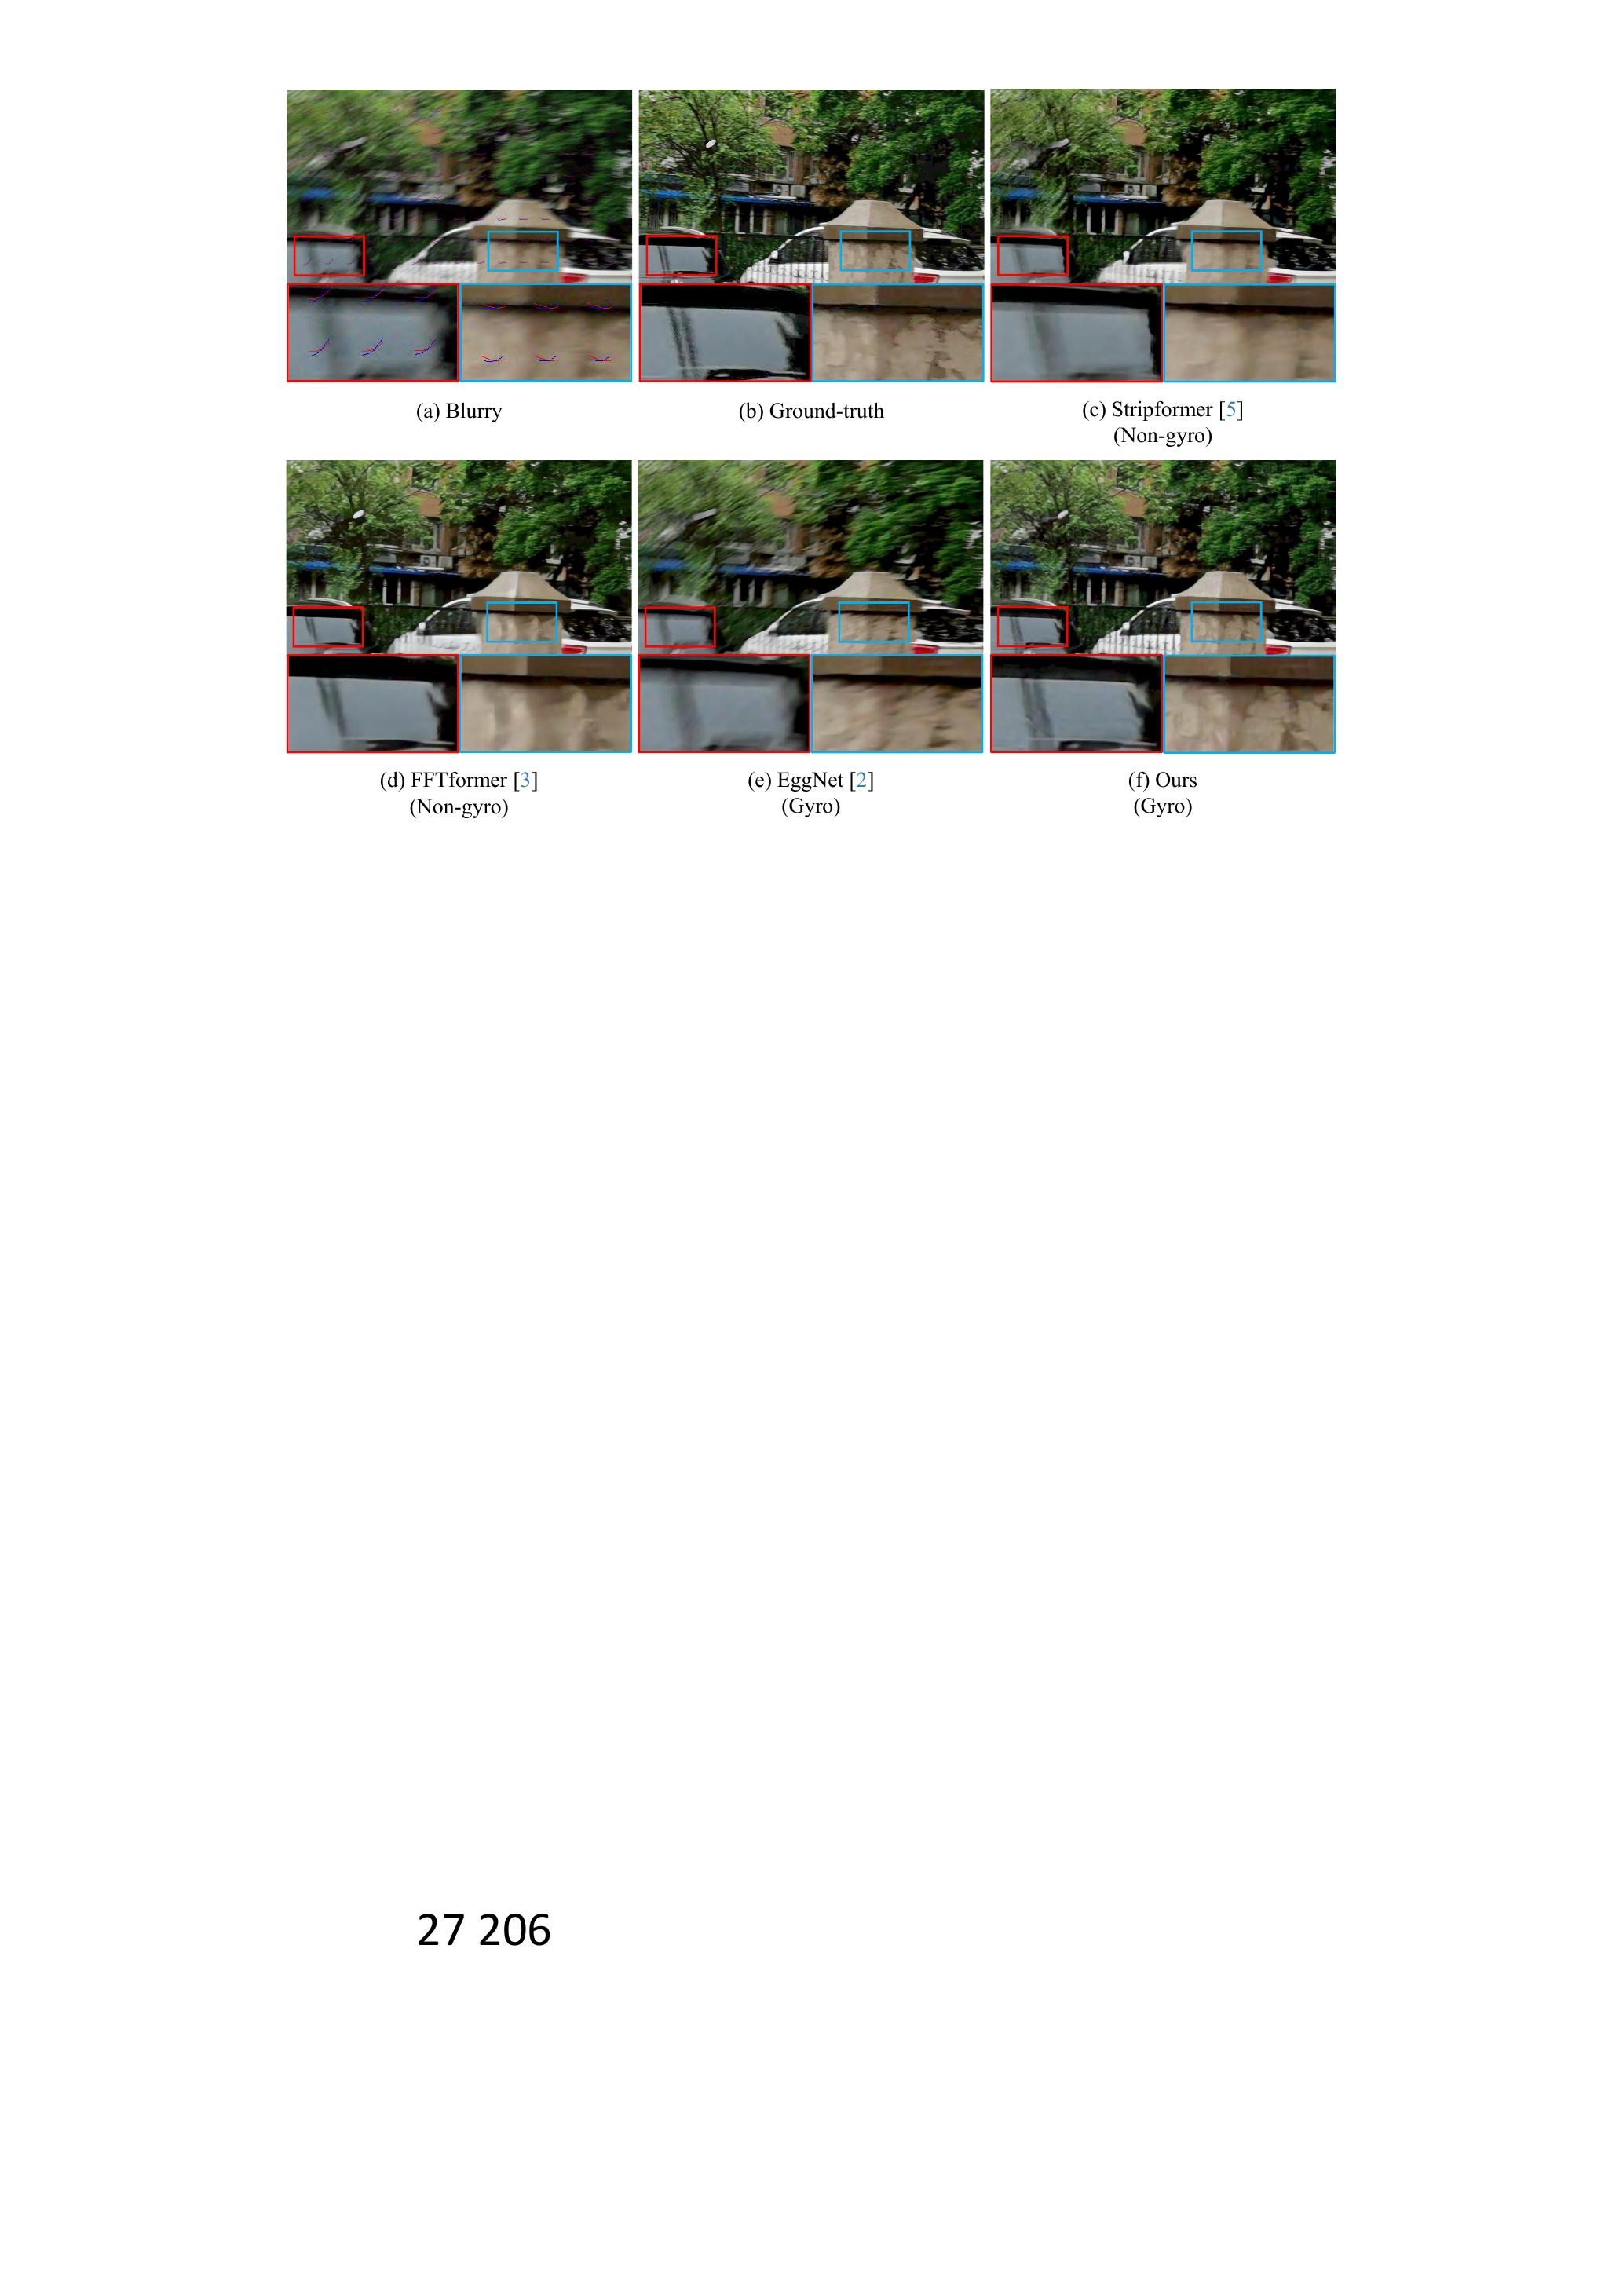}
\caption{Additional qualitative results on \SynthDataName{}. In (a), red lines and blue lines visualize erroneous camera motion field and accurate camera motion field respectively.}
\label{fig:qualitative_synth_supple_3}
\end{figure*}

\begin{figure*}[t]
\centering
\includegraphics[width=\linewidth]{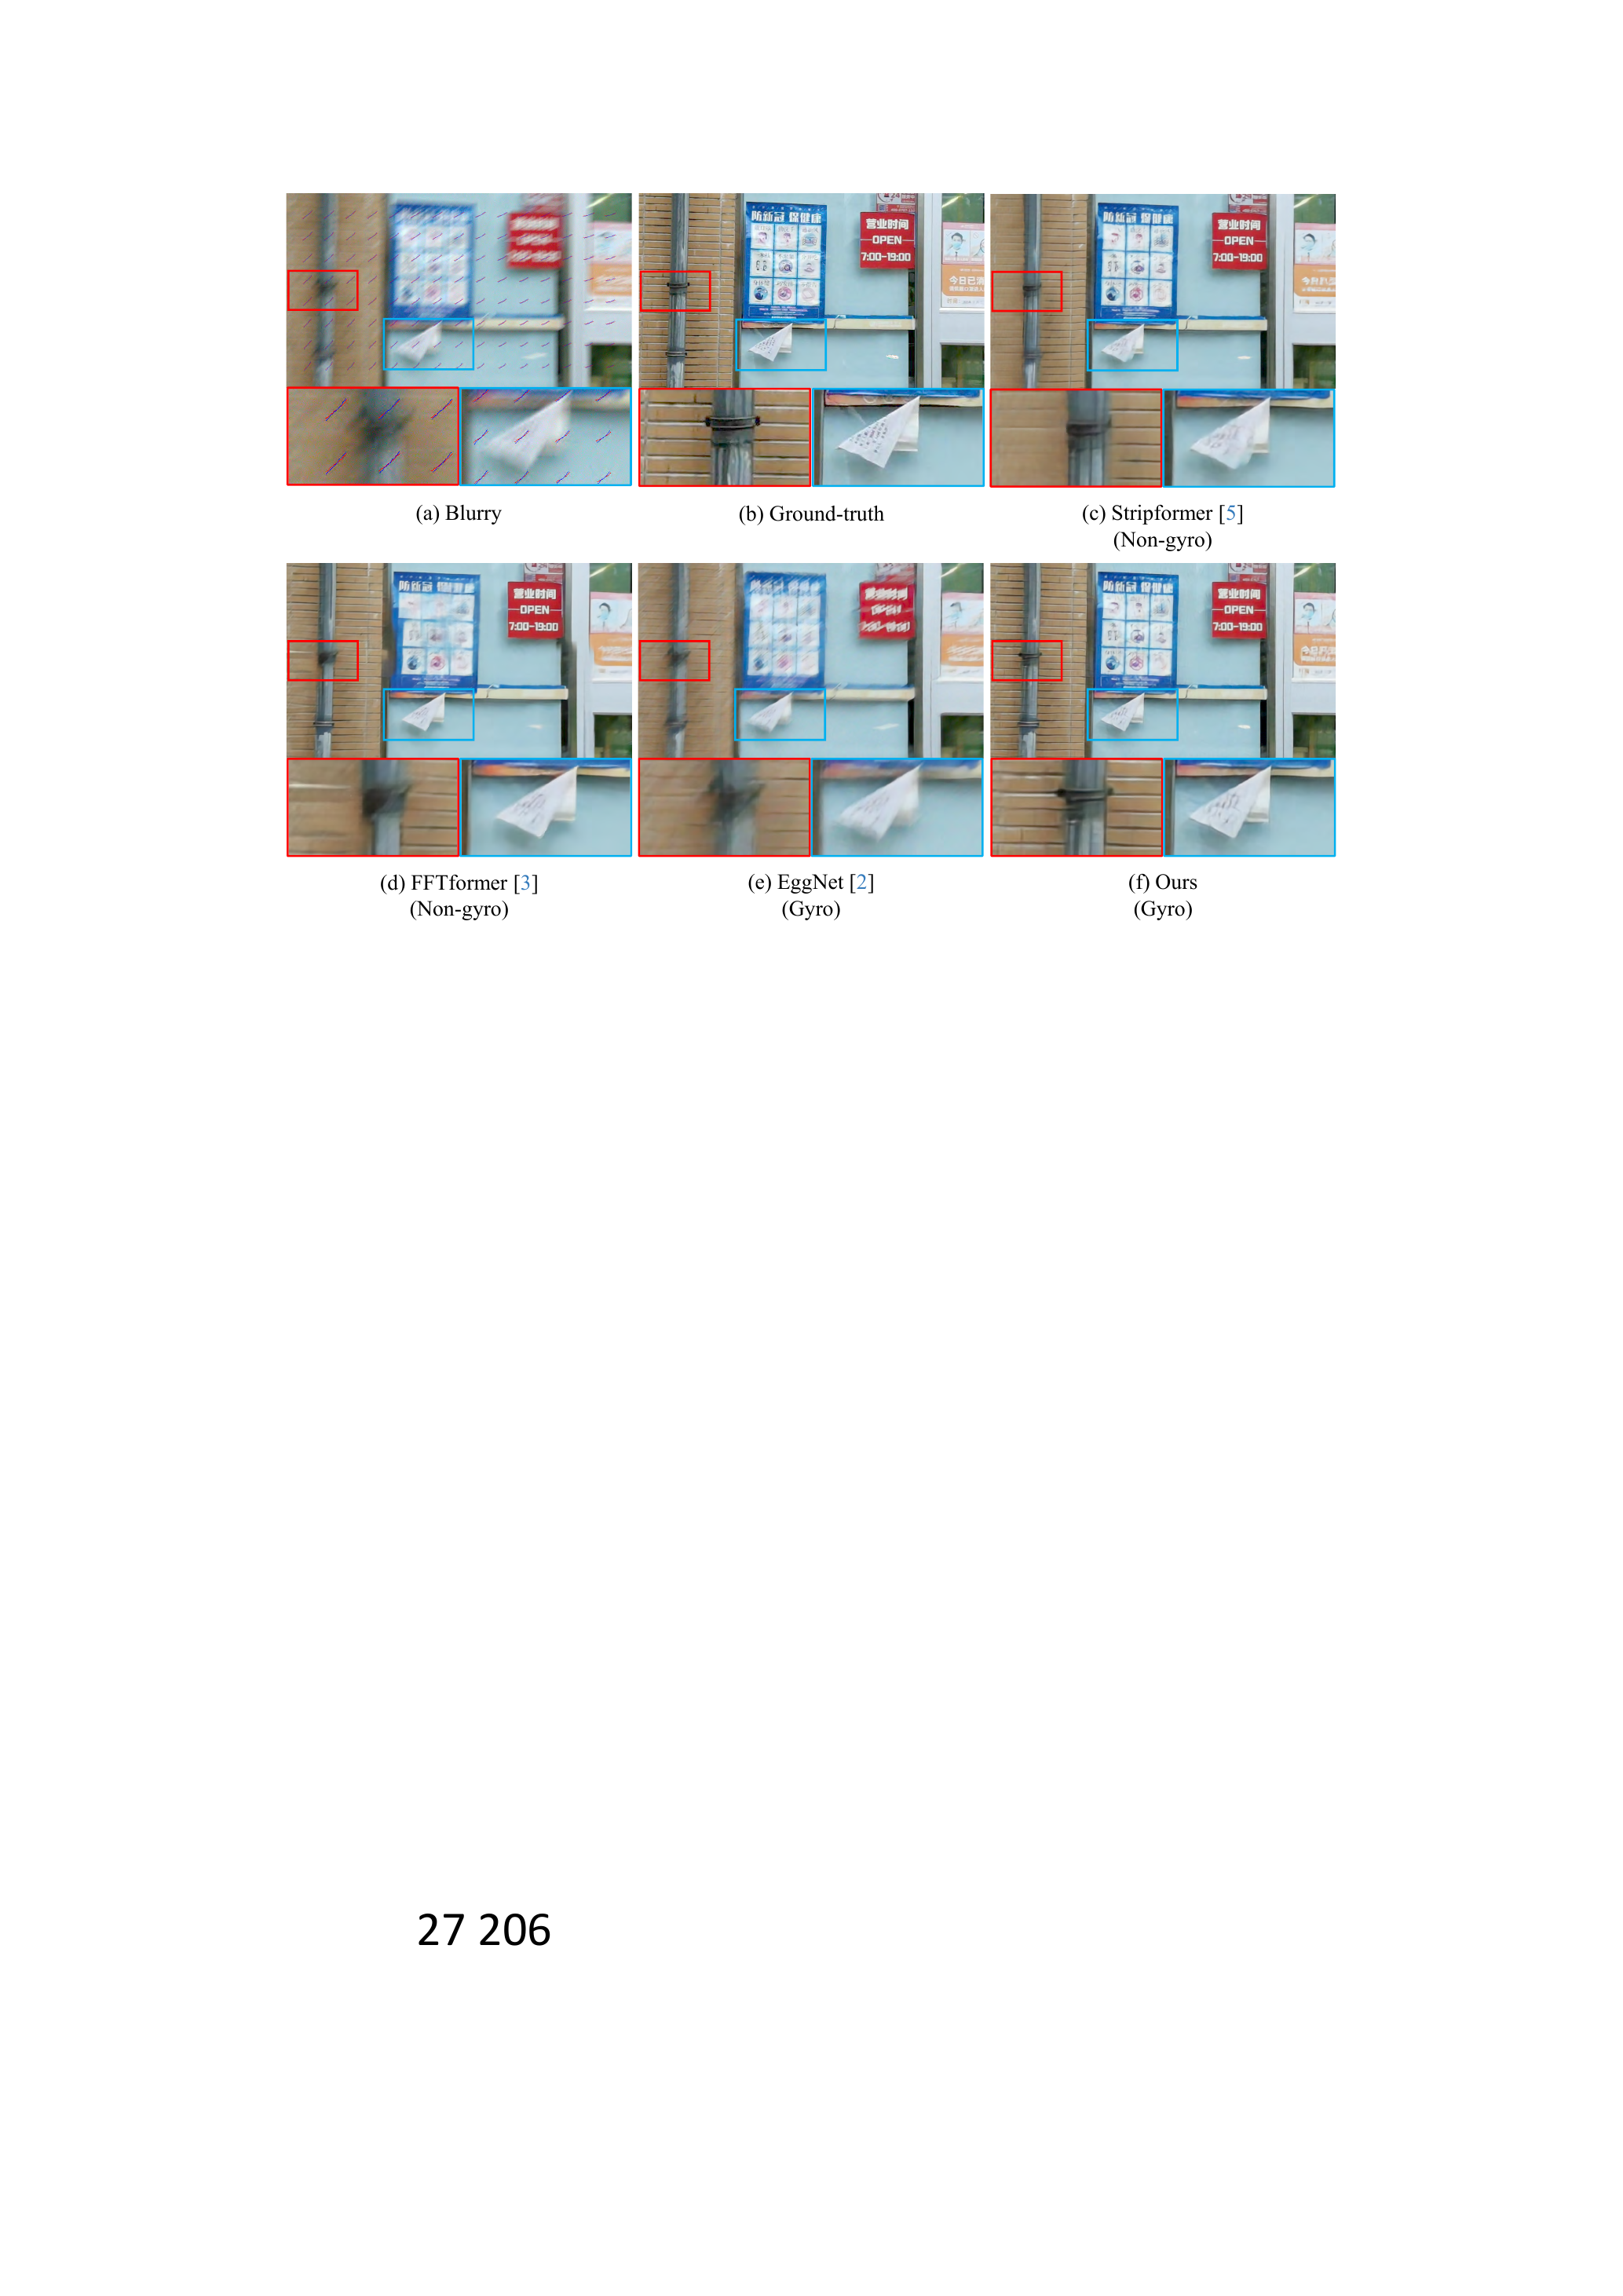}
\caption{Additional qualitative results on \SynthDataName{}. In (a), red lines and blue lines visualize erroneous camera motion field and accurate camera motion field respectively.}
\label{fig:qualitative_synth_supple_4}
\end{figure*}

\begin{figure*}[t]
\centering
\includegraphics[width=0.9\linewidth]{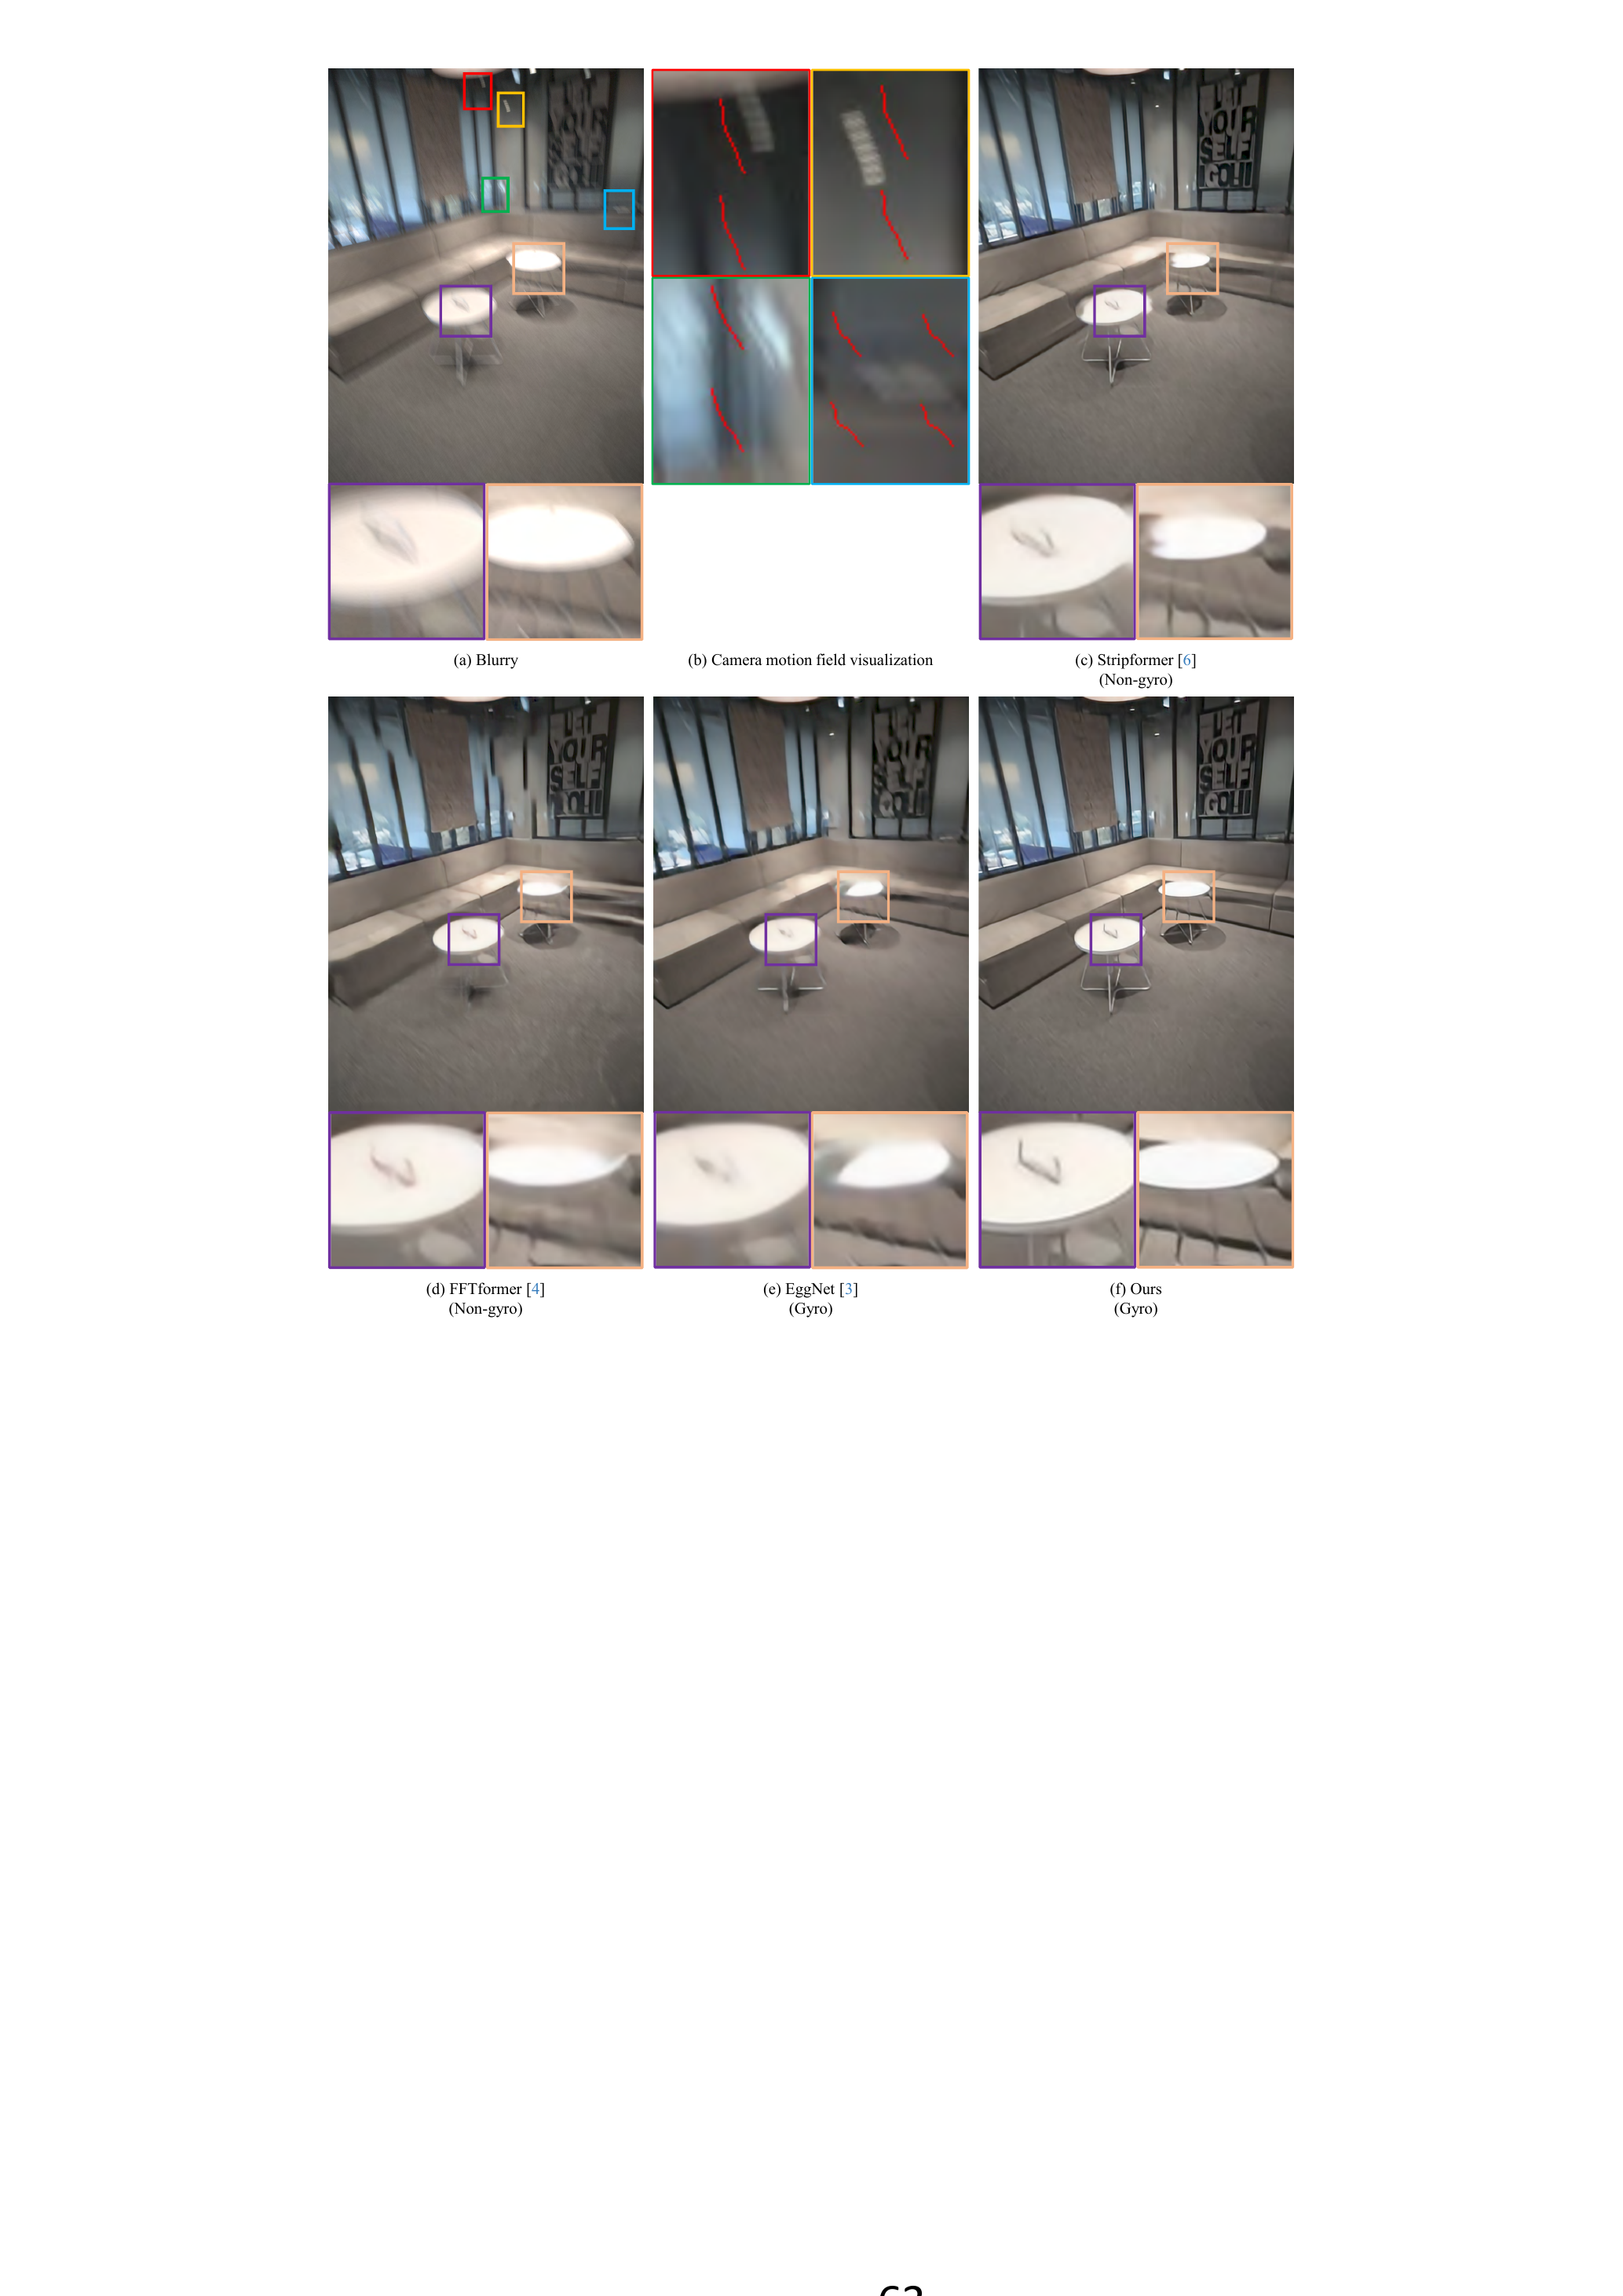}
\caption{Additional qualitative results on \RealDataName{}. In (b), red lines visualize real-world camera motion field.}
\label{fig:qualitative_real_supple_1}
\end{figure*}

\begin{figure*}[t]
\centering
\includegraphics[width=0.9\linewidth]{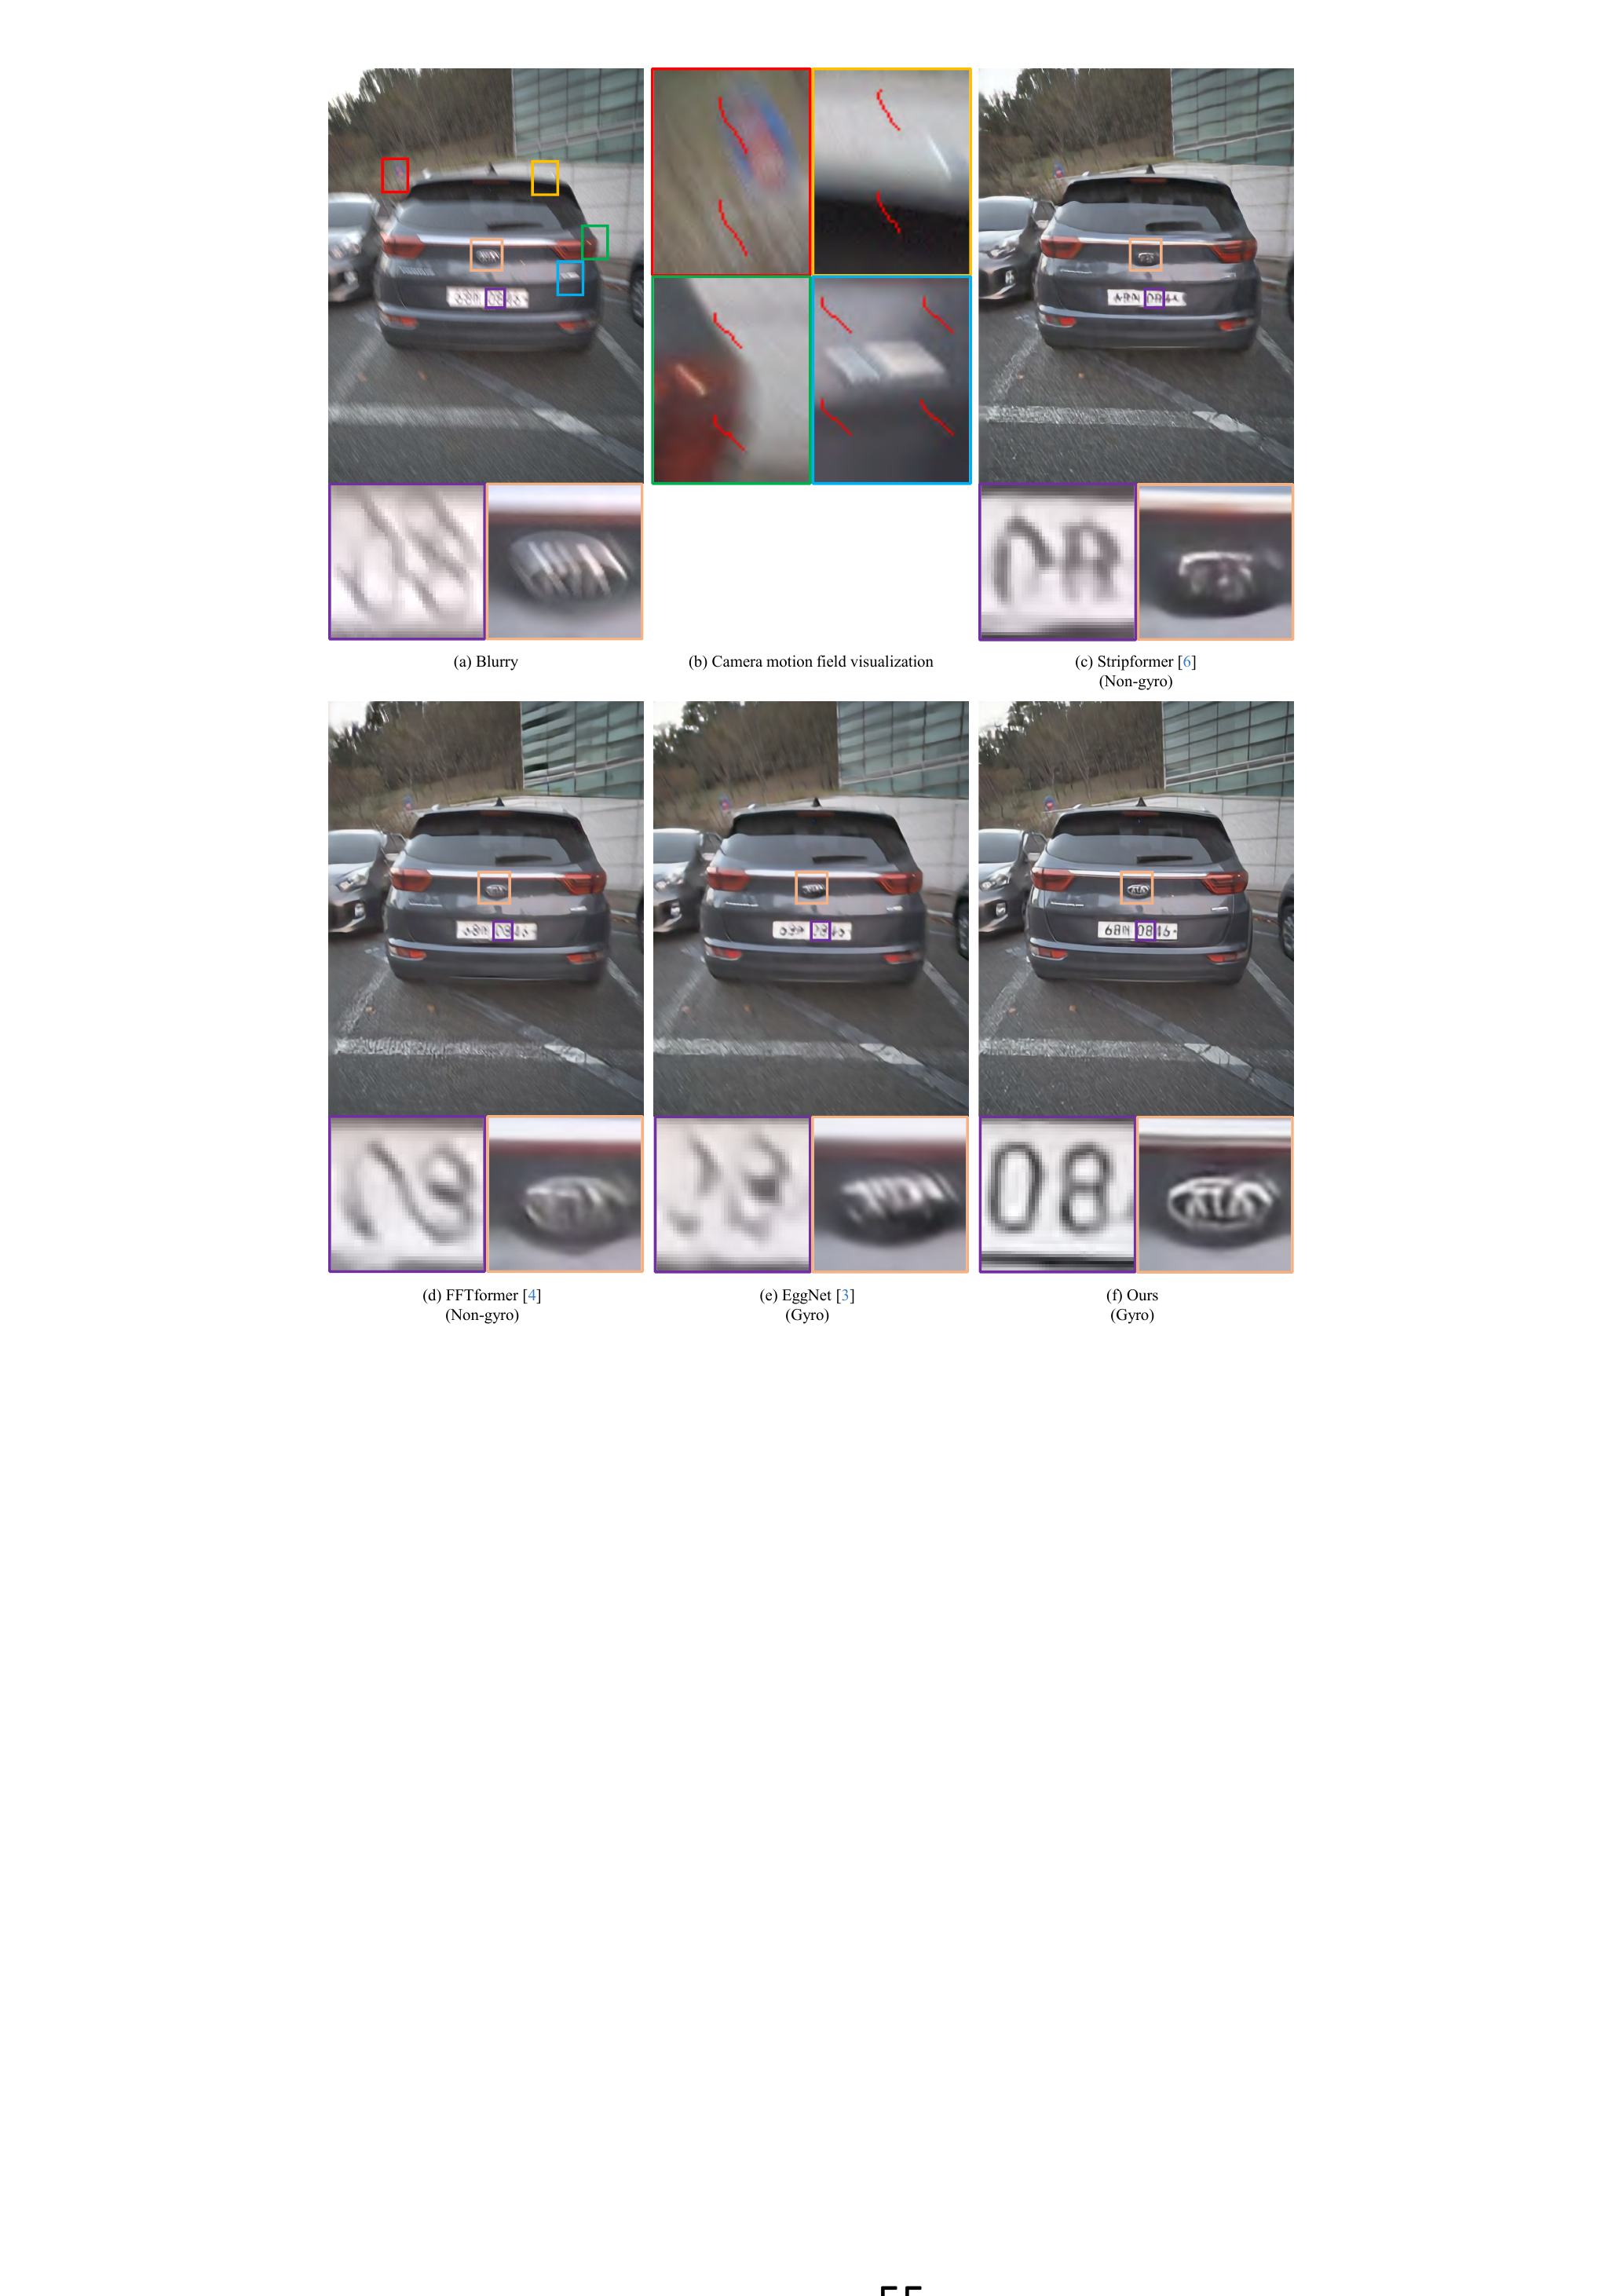}
\caption{Additional qualitative results on \RealDataName{}. In (b), red lines visualize real-world camera motion field.}
\label{fig:qualitative_real_supple_2}
\end{figure*}

\begin{figure*}[t]
\centering
\includegraphics[width=0.9\linewidth]{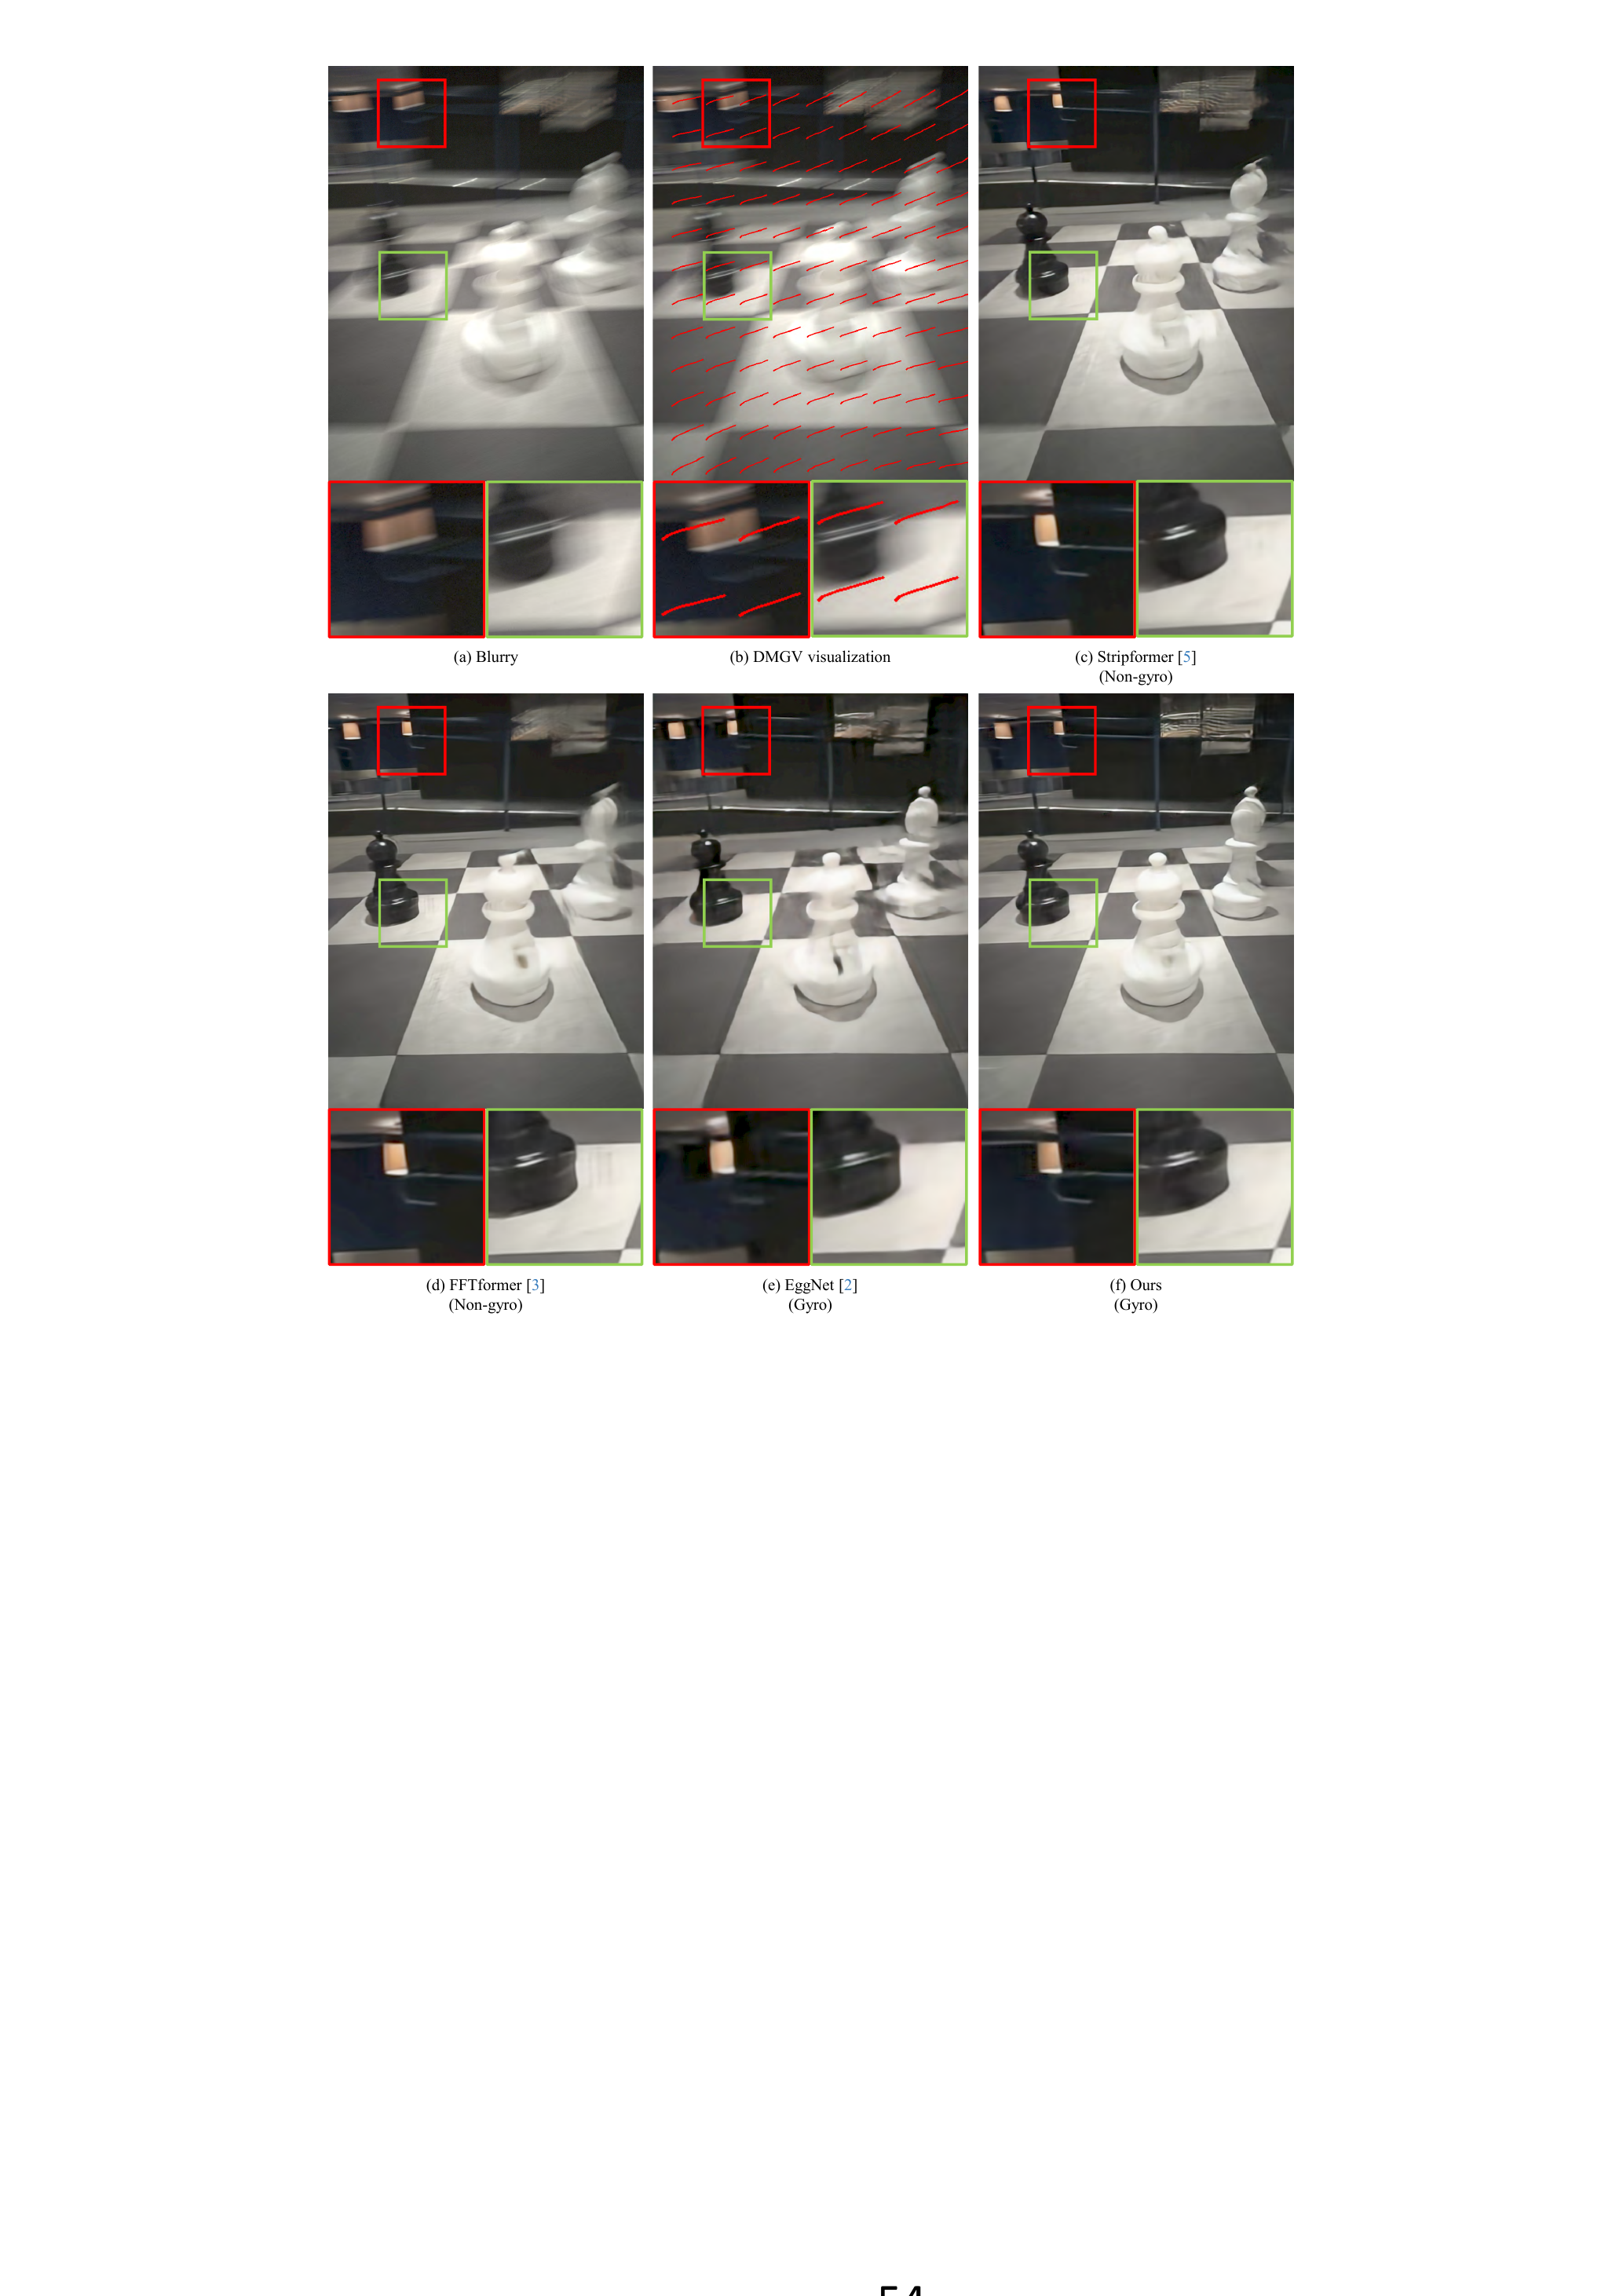}
\caption{Additional qualitative results on \RealDataName{}. In (b), red lines visualize real-world camera motion field.}
\label{fig:qualitative_real_supple_3}
\end{figure*}

\begin{figure*}[t]
\centering
\includegraphics[width=\linewidth]{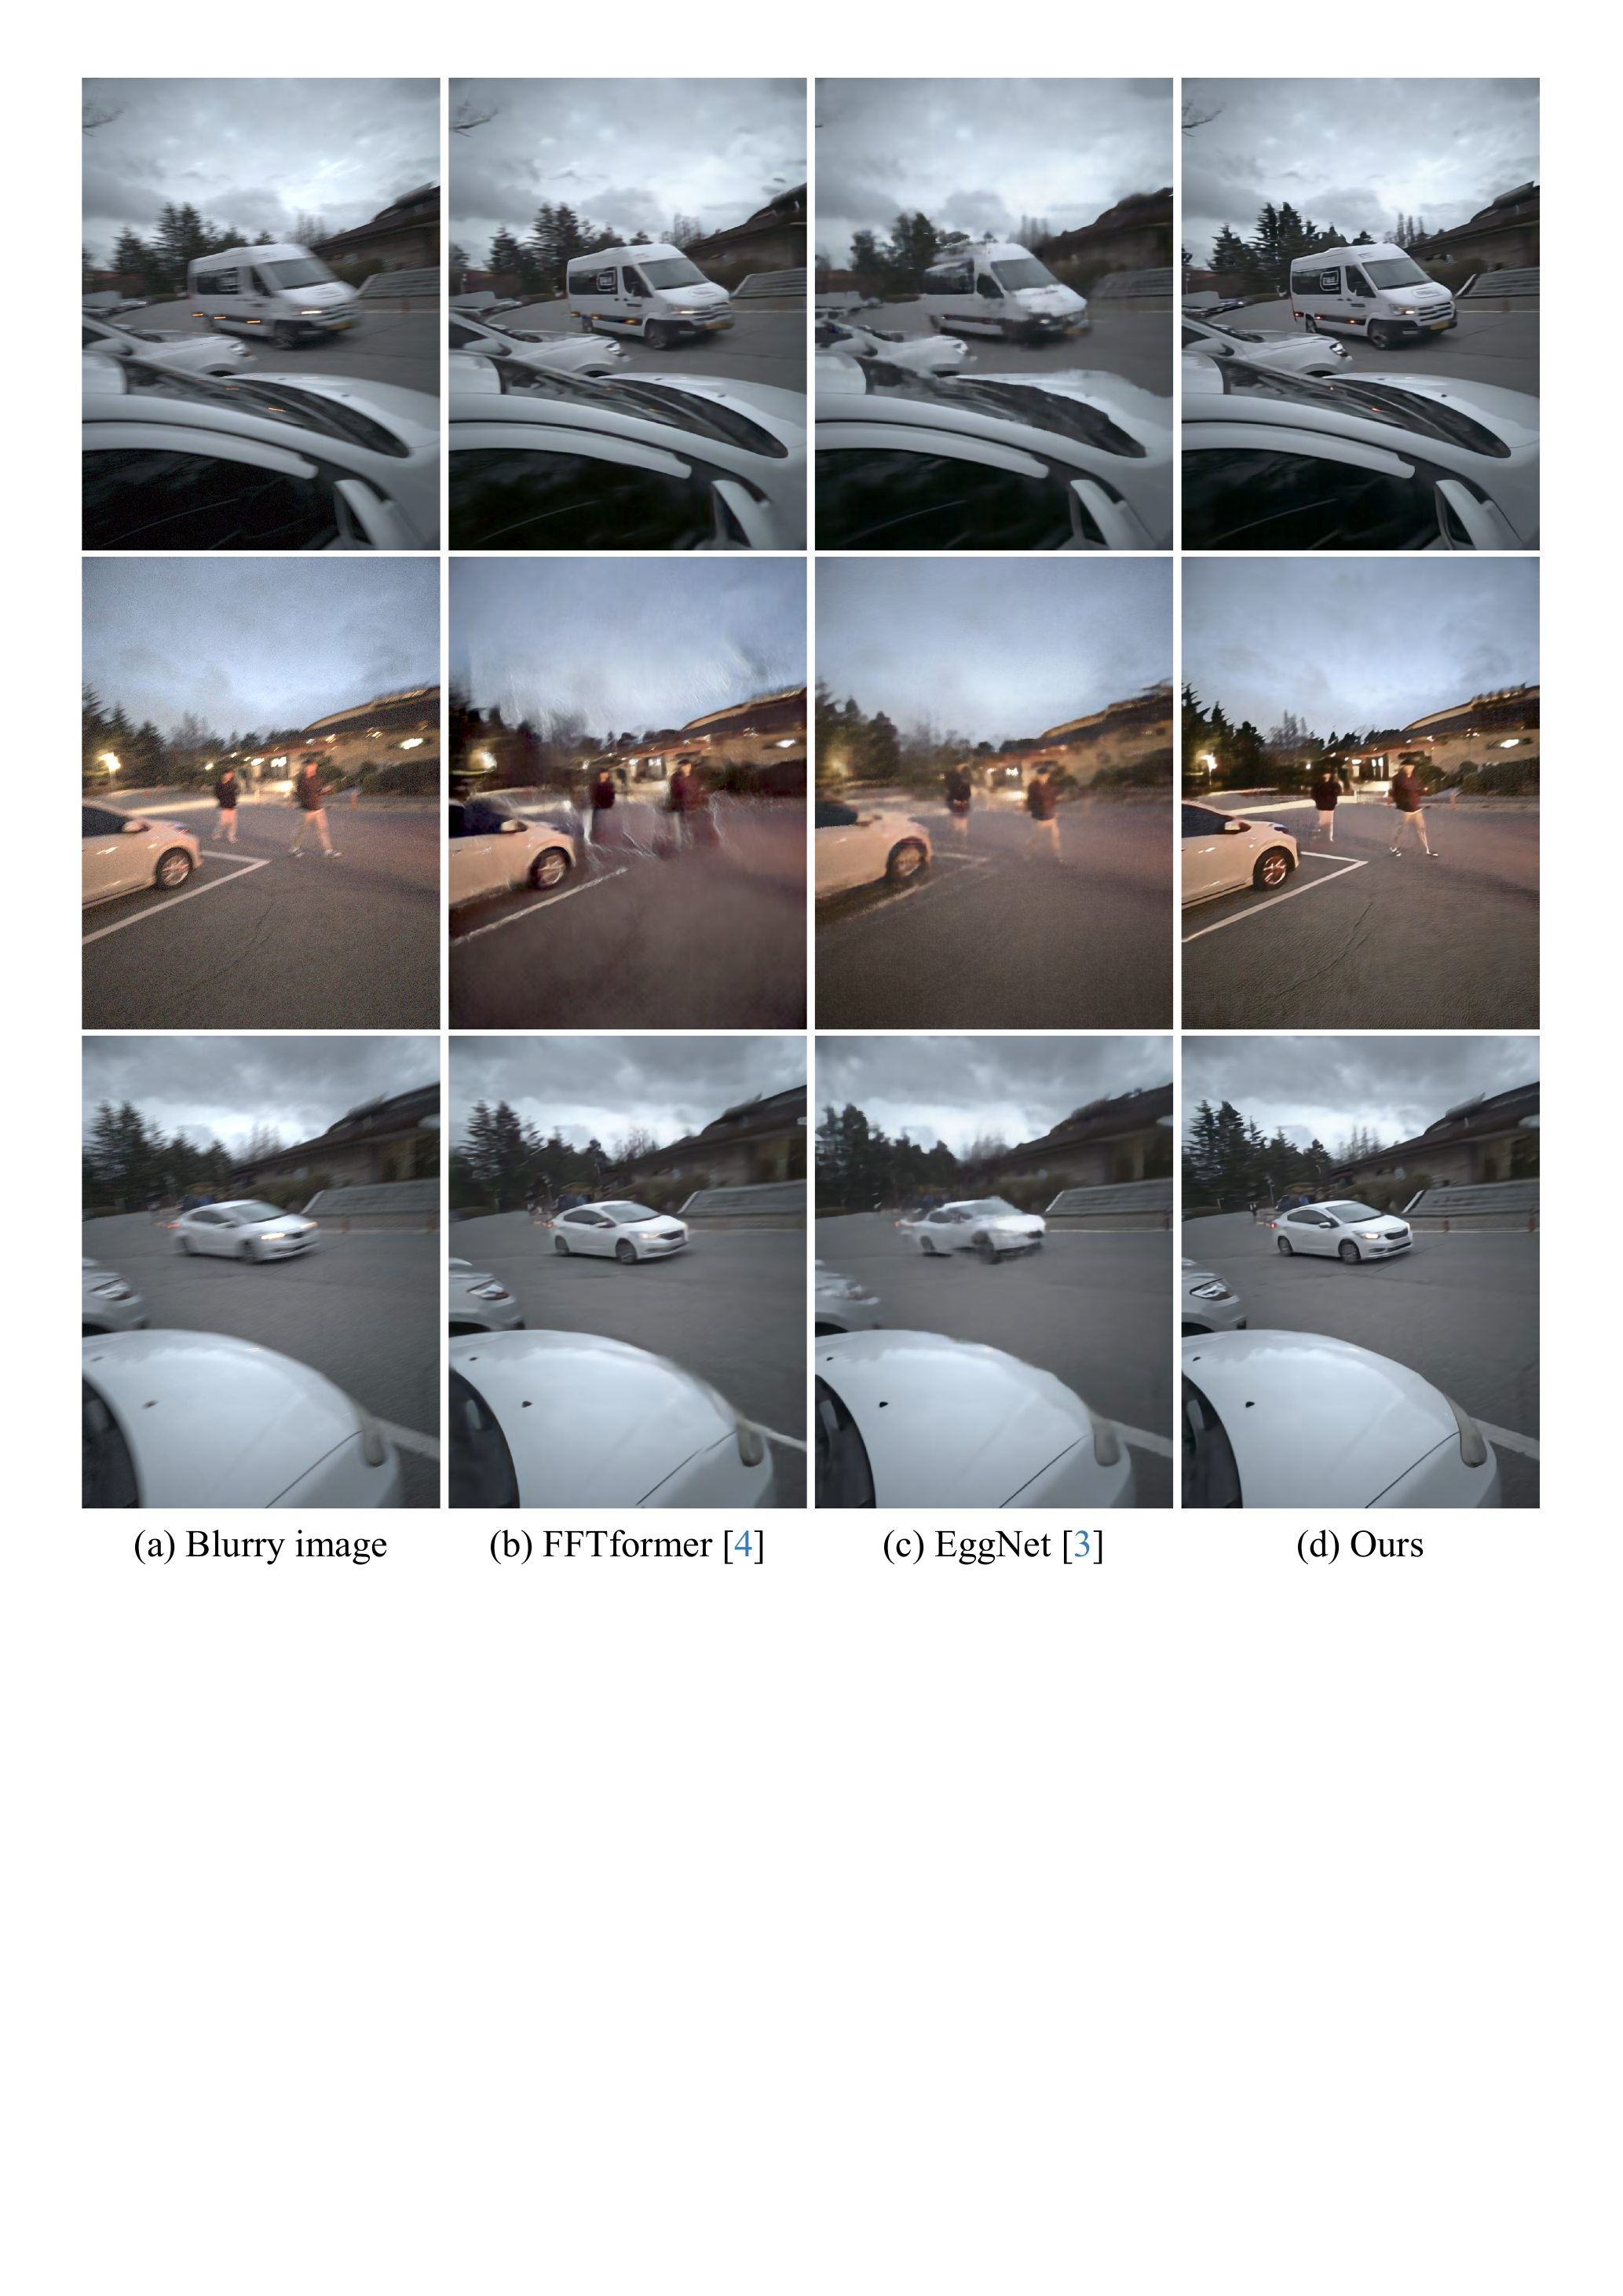}
\caption{Additional qualitative results on real-world image with moving objects.}
\label{fig:moving_object_real_supple}
\end{figure*}
