# Supplementary material for: Gyro-based Neural Single Image Deblurring
Source: arXiv:2404.00916 source file (2025-04-04)
Supplement: Supplementary file 2 [file fig_rot_cen_visualization_supple.pdf]

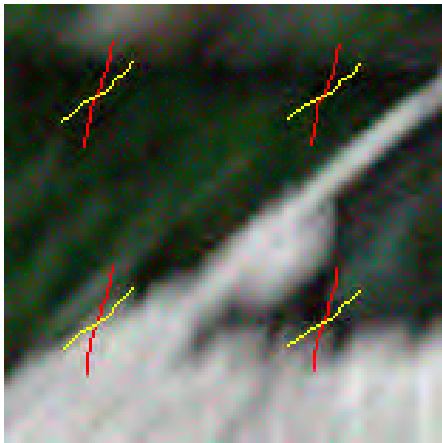

(a) Blurry

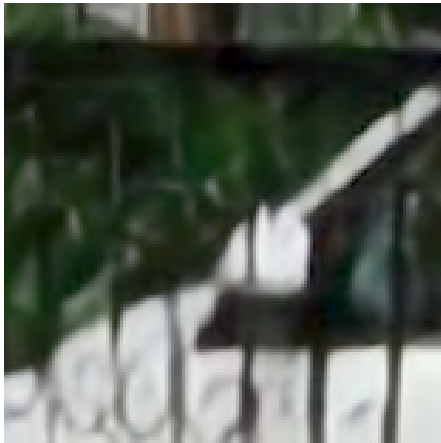

(b) No error

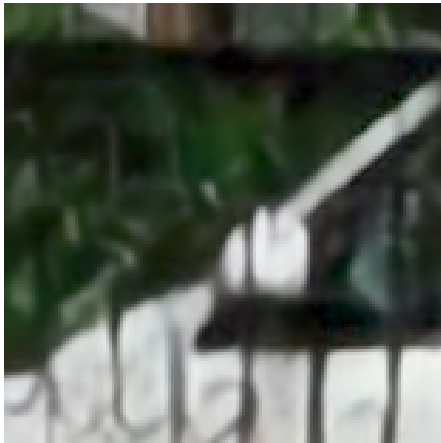

(c) Error  
(1000, 1000)

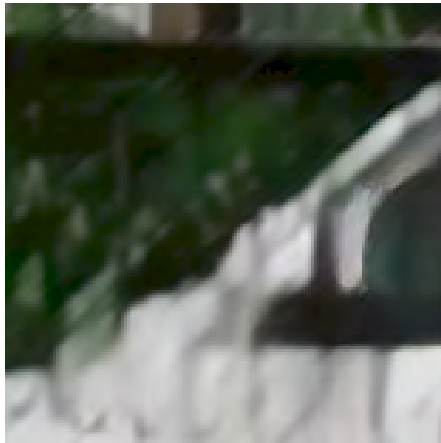

(d) FFTformer [3]
